# Supplementary material for: VerilogCoder: Autonomous Verilog Coding Agents with Graph-based Planning and Abstract Syntax Tree (AST)-based Waveform Tracing Tool
Source: arXiv:2408.08927 source file (2025-03-05)
Supplement: Supplementary file 1 [file VerilogCodeAgent_appendix_arXiv.pdf]

# VerilogCoder Technical Appendix

**Chia-Tung Ho, Haoxing Ren, Brucek Khailany**

NVIDIA Research
chiatungh@nvidia.com, haoxingr@nvidia.com, bkhailany@nvidia.com

## Prompts of Task Planning

We present the prompts of the agents for task planning as follows: (1) high-level planner agent, (2) circuit signal, transition, and example extraction agent, and (3) task-driven circuit relation graph retrieval agent. Figure 1 shows the prompt used to decompose the task into manageable sub-tasks in JSON format. For creating the Task and Circuit Relation Graph, the circuit signal, transition, and example extraction agent extracts the circuit-related signals using the prompt in Figure 2. Lastly, after constructing the Task and Circuit Relation Graph, the task-driven circuit relation graph retrieval agent retrieves detailed signal descriptions for each sub-task. Figure 3 shows the prompt for the task-driven circuit relation graph retrieval agent to retrieve information for each sub-task.

**High-level planner agent prompt template**

```
You are a Verilog RTL designer that can break down complicated implementation into subtasks implementation plans.

[Example Begin]
{VerilogExamples}
[Example End]

[Target Problem]
### Problem

{ModuleDescription}

[Instruction]
Let's think step by step.
Based on the Problem description, set up a sequential implementation plans. Each subtask should focus on implement only one signal at a time.
Extract the corresponding source contexts in the [Target Problem] section of each subtask into the 'source' field.
The task id number indicates the sequential orders. Return the subtasks in json format as below.
```json
{ "subtasks": [
            {
              "id": "1",
              "content": "task description 1",
              "source": "source 1"
            },
            {
              "id": "2",
              "content": "task description 2",
              "source": "source 2"
            },
            {
              "id": "3",
              "content": "task description 3",
              "source": "source 3"
            },
            ...
          ]
}
```

[Rules]
Make sure the task plans satisfy the following rules! Do not make the plans that violate the following rules!!!
- Make a plan to define the module with its input and output first.
- Do not plan the implementation of logic or signal from the input ports.
- There is test bench to test the functional correctness. Do not plan generating testbench to test the generated verilog code.
- Don't make a plan only with clock or control signals. The clock or control signals should be planned with register or wire signal.
- Don't make a plan on implementing the signal or next state logics which are not related to the module outputs.
- For module related to Finite State Machine (FSM), try to determine the number of states first and then make the plan to implement FSM.
- For module related to Finite State Machine or Moore State Machine, if the state or current_state is an input port signal of the module, You must Do Not implement the state flip-flops for state transition in TopModule.
```

Figure 1: The prompt template of high-level planner agent. The blue texts are variables and can be replaced according to various task descriptions.

**Circuit signal, transition, and example extraction agent prompt template**

````
You are a Verilog RTL designer that identify the signals, state transition description, and signal example contents.

[Module Description]
{ModuleDescription}

[Instruction]
Extract the signal and its description, state transition description, and signal example contents in the json format.
The return format need to follow ```json and ``` format.
```json
{
  "signal": ["<signal1 name>: <signal1 description>", "<signal2 name>: <signal2 description>", ...], # list of strings
  "state_transitions_description": [<state_transition_line1>, <state_transistion_line2>, ...], # list of strings
  "signal_examples": [<text1>, <text2>, ...], # list of strings
}
```

[Rules]:
- You must extract the signals and all signal examples in the description!
- Do not implement the verilog code. Do not change the original description and text.
- Do not change the state_transition format when extracting to 'state_transitions_description'.
- If the state_transition is represented as K-map table, you need to extract the row or column values with their corresponding row or column signals.
- Do not add signal examples if there is no examples in the module description.
````

Figure 2: The prompt template of circuit signal, transition, and example extraction agent. The blue texts are variables and can be replaced according to various task descriptions.

**Task-driven circuit relation graph retrieval agent prompt template**

````
You are a top-tier Verilog expert with experience in retrieving required information for the following task using retrieve_additional_plan_information_tool.
[Module Description]:
{ModuleDescription}

[Current Task Description]:
```
{CurrentTask}
```

Let's think step by step.
1. Set BFS_retrival_level=2.
2. Use retrieve_additional_plan_information_tool to retrieve the required information. The rules for covering the task are below.
  - have the signal mentioned in the task
  - Must have the signal example if there are any related to the task
3. Increase the BFS_retrival_level by 1 and repeat the step 2. BFS_retrival_level should not exceed 10.
  - If the task is well covered by the retrieved information or no more retrieved information available, go to Step 4.
4. Compile the node names and descriptions which covers the task from the BFS result.
  - You must remove the signal which is not mentioned in the task. Make the related information short and be able to cover the task need.
  - Must include the signal example (Type: SignalExample) if the signal is mentioned in the task.

Return the Task and retrieved related information from retrieve_additional_plan_information_tool.
If there is no retrieved related information needed for the Task, just return the Task.
The return format is below.
```
{CurrentTask}

Retrieved Related Information:
Info 1
Info 2
...
```
After the return format, reply TERMINATE to end.
````

Figure 3: The prompt template of task-driven circuit relation graph retrieval agent. The blue texts are variables and can be replaced according to various task descriptions.

## Prompts of Verilog code implementation

We present the prompts for the code agent and the debug agent for Verilog code implementation task. The code agent's prompt is illustrated in Figure 4. The code agent completes the current sub-task by considering the examples, module description, and partial Verilog code from previous tasks. Figure 5 shows the prompt template for the debug agent. This prompt includes the module description and the completed Verilog code from the code agent. The agent must run the simulator and debug until the module functions correctly.

**Code agent prompt template**

```
You are a Verilog RTL designer that only writes code using correct Verilog syntax based on the task definition.

[Example Begin]
{VerilogExamples}
[Example End]

[Module Description]
{ModuleDescription}

[Previous Module Implementation]
```verilog
{PreviousTaskOutput}
```

[Current SubTask]
{Task}

[Hints]:
- For implementing kmap, you need to think step by step. Find the inputs corresponding to output=1, 0, and don't-care for each case. Categorized them and find if there are any combinations that can be simplify.

[Rules]:
- Only write the verilog code for the [Current SubTask]. Don't generate code without defined in the [Current SubTask].
- Don't change or modify the code in [Previous Module Implementation].
- Return the written verilog log code with Previous Module Implementation.
- Declare all ports and signals as logic.
- Don't use state_t to define the parameter. Use `localparam` or Use 'reg' or 'logic' for signals as registers or Flip-Flops.
- Don't generate duplicated signal assignments or blocks.
- Define the parameters or signals first before using them.
- Not all the sequential logic need to be reset to 0 when reset is asserted.
- for combinational logic, you can use wire assign (i.e., assign wire = a ? 1:0;) or always @(*).
- for combinational logic with an always block do not explicitly specify the sensitivity list; instead use always @(*).
- For 'if' block, you must use begin and end as below.
  [if example]
  if (done) begin
    a = b;
    n = q;
  end
  [if example end]
```

Figure 4: The prompt template of code agent. The blue texts are variables and can be replaced according to various task descriptions.

**Debug agent prompt template**

```
You are a Verilog RTL designer that only writes code using correct Verilog syntax and verify the functionality.
You need to run the verilog_simulation_tool to make sure the functional correctness before TERMINATE.

[Target Module Description]
### Problem
{ModuleDescription}

### Completed Verilog Module
```verilog
{CompletedVerilogCodeModule}
```


[Instructions]:
1. Use the verilog_simulation_tool to verify the syntax and functional correctness of the Completed Verilog Module.
2. Use the waveform_trace_tool to trace the waveform of functional incorrect signals by inputting the verilog_simulation_tool result.
3. Debug the waveform and verilog source code and find out the signals need to be corrected.
4. Repeat above steps until pass the syntax and functional check.

[Constraints]:
- Do not use typedef enum in the verilog code.
- There is test bench to test the functional correctness. You don't need to generate testbench to test the generated verilog code.
- Do not use $display or $finish in the module implementation.
- You can not modify the testbench.
- Declare all ports as logic; use wire or reg for signals inside the block.
- Don't use state_t. Use 'reg' or 'logic' for signals as registers or Flip-Flops.
- for combinational logic, you can use wire assign or always @(*).
- for combinational logic with an always block do not explicitly specify the sensitivity list; instead use always @(*)
- Don't generate duplicated signal assignments or blocks.
```

Figure 5: The prompt template of debug agent. The blue texts are variables and can be replaced according to various task descriptions.

# Inconsistent Specification and Reference Design Module in the VerilogEval-Human v2 Benchmark

We observed approximately 7% inconsistency between specifications and reference design modules in the VerilogEval-Human v2 benchmark, available at https://github.com/NVlabs/verilog-eval. Below, we list common inconsistencies between specifications and reference design modules across a few representative cases.

**Module port definition or wrong combination logic description** Figure 6 illustrates representative cases of this type of inconsistency. In the case of Prob134_2014_q3c, the description omits the input clk, which is present in the reference design module. For Prob045_edgedetect2 description, the output port anyedge is defined with the wrong direction. In Prob074_ece241_2014_q4, the output z is defined as the result of a three-input XNOR gate, but the reference design module implements a NOR gate for the output z.

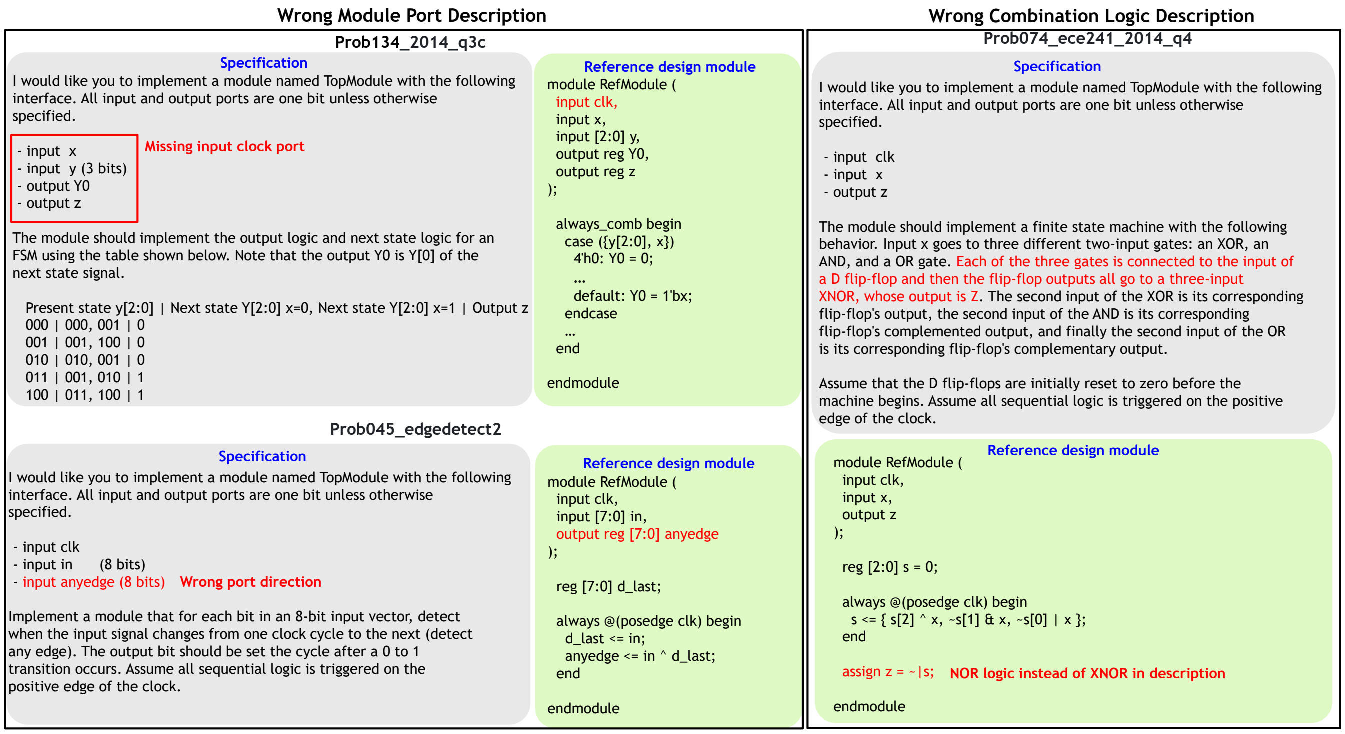


Figure 6: The examples of module port definition or wrong combination logic description. Prob134_2014_q3c and Prob045_edgedetect2 have wrong port description. Prob074_ece241_2014_q4 has wrong combination logic description of output z.

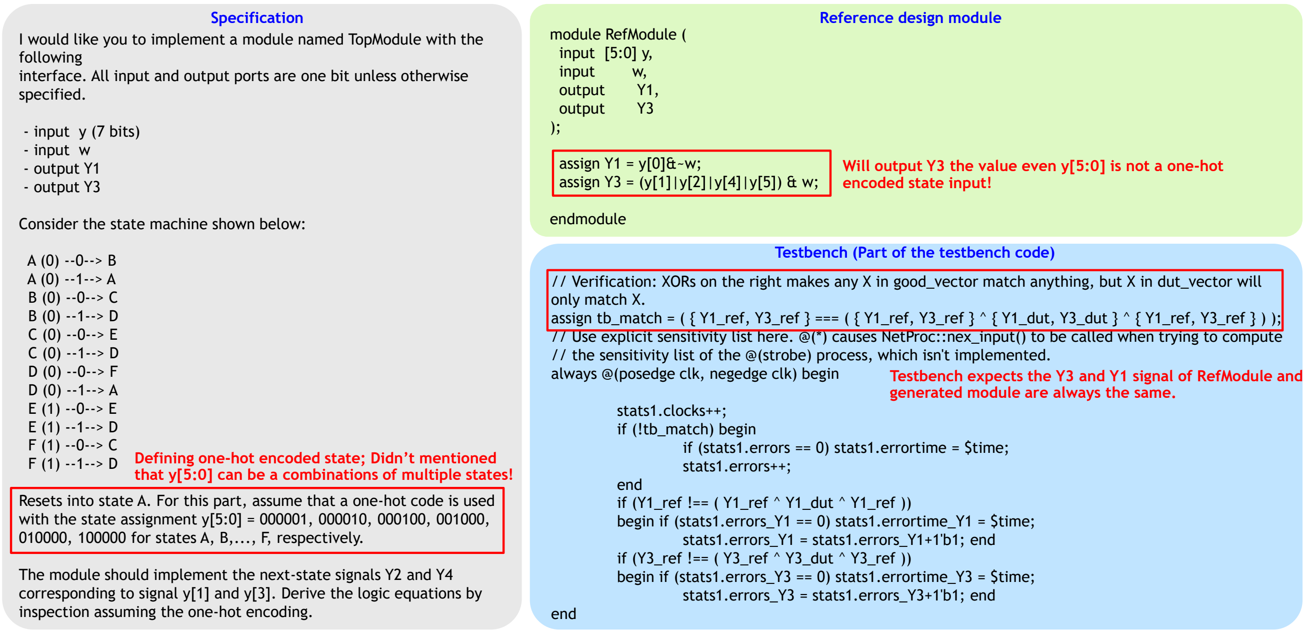


Figure 7: An example of State condition of finite state machine. In Prob099_m2014_q6c, it define one-hot encoded state machine, but failed to provide the information of the input y[5:0] port could be a combination of multiple one-hot encoded states and the testbench expects the Verilog module to generate valid output signals.

**State condition of finite state machine** In some cases, the descriptions define a one-hot encoded Moore state machine but fail to provide information indicating that the input state port could be a combination of multiple one-hot encoded states. The testbench, however, expects the Verilog module to generate valid output signals, which creates confusion when large language models attempt to write a functionally correct Verilog module, especially when debugging a waveform with the input state port containing multiple one-hot encoded states. For instance, Figure 7 highlights the inconsistency between the description and the reference design module concerning the input state (i.e., y[5:0]) port and the expected behavior of the output ports in Prob099_m2014_q6c.

**Updated Specification**

```
I would like you to implement a module named TopModule with the
following
interface. All input and output ports are one bit unless otherwise
specified.

 - input  y (6 bits)
 - input  w
 - output Y1
 - output Y3

Consider the state machine shown below:

  A () --0--> B
  A () --1--> A
  B () --0--> C
  B () --1--> D
  C () --0--> E
  C () --1--> D
  D () --0--> F
  D () --1--> A
  E () --0--> E
  E () --1--> D
  F () --0--> C
  F () --1--> D

Resets into state A. For this part, assume that a one-hot code is used
with the state assignment y[5:0] = 000001, 000010, 000100, 001000,
010000, 100000 for states A, B,..., F, respectively.
Here,the y[5:0] could can be a combinations of multiple states above.
The implemented module is expected to response the state bit.
For example, when y[5:0] = 6'b000110, y[2] == 1, y[1] == 1, the states
include B, and C states.

The module should implement the next-state signals Y1 and Y3
corresponding to signal y[1] and y[3]. Derive the logic equations by
inspection assuming the one-hot encoding.
```

Provide the example of y[5:0] could be a combinations of multiple states and the output signals are expected to response.

**GPT-4 Turbo without agent-based approach: functional incorrect Verilog module**

```
module TopModule
(
  input  logic [5:0] y,
  input  logic w,
  output logic Y1,
  output logic Y3
);

  // Combinational logic for state transitions
  always @(*) begin
    Y1 = ((y[1] & ~w) | (y[3] & ~w)); // Next state of B (y[1]) is either C (y[2]) or D (y[3]) based on 'w'
    Y3 = ((y[1] & w) | (y[2] & w) | (y[4] & w) | (y[5] & ~w)); // Next state of D (y[3]) is either A (y[0]), B (y[1]), E (y[4]) or F (y[5]) based on 'w'
  end

endmodule
```

**VerilogCoder: functional correct Verilog module**

```
module TopModule
(
  input  logic [5:0] y,
  input  logic       w,
  output logic       Y1,
  output logic       Y3
);

  // Logic for next-state signal Y1
  assign Y1 = y[0] & ~w;

  // Logic for next-state signal Y3
  assign Y3 = (y[1] & w) | (y[2] & w) | (y[4] & w) | (y[5] & w);

endmodule
```

Figure 8: (1) The updated description for Prob099_m2014_q6c, (2) Functional incorrect Verilog module generated by GPT-4 Turbo without agent-based approach with the updated description for Prob099_m2014_q6c, and (3) Functional correct Verilog module generated by VerilogCoder.

We ran GPT-4 Turbo without an agent-based approach using the corrected prompts (i.e., approximately 7% of the VerilogEval-Human v2 benchmark) but did not observe obvious improvement in generating functionally correct Verilog modules. Figure 8 shows the failed Verilog module implementations by GPT-4 Turbo without the agent-based approach, as well as by the proposed VerilogCoder, on Prob099_m2014_q6c with the corrected description. Consequently, we continue to use the experimental data from prior work (Pinckney et al., 2024) for comparison in the Main Results. We are collaborating with the authors of VerilogEval-Human v2 (Pinckney et al., 2024) to update the benchmark at https://github.com/NVlabs/verilog-eval. These updates will be available to the public shortly.

## Examples of Fixing Functionality of Verilog Module

Here, we demonstrate an example of fixing the functionality of a Finite State Machine module for receiving serial input data. The debugging trace of the Debug Agent, which leverages the developed AST-based waveform tracing tool to fix functional errors, is shown below.

**user (to chat_manager):**
You are a Verilog RTL designer that only writes code using correct Verilog syntax and verify the functionality.
[Target Module Description]
### Problem
I would like you to implement a module named TopModule with the following
interface. All input and output ports are one bit unless otherwise
specified.
 - input  clk
 - input  in
 - input  reset
 - output out_byte (8 bits)
 - output done
In many (older) serial communications protocols, each data byte is sent along
with a start bit and a stop bit, to help the receiver delimit bytes from the
stream of bits. One common scheme is to use one start bit (0), 8 data bits, and
1 stop bit (1). The `in` stays at logic 1 when nothing is being transmitted.
The FSM should start to receive the following 8 data bits right after detect the
start bit (0). Design a finite state machine that will identify when bytes have been
correctly received when given a stream of bits. It needs to start to receive the data
right away when the start bit (0) occurs, receive the consecutive all 8 data bits,
then verify that the stop bit (1) was correct of `in`. `done` is set to 1 after verify
the stop bit (1), otherwise, it will be remain 0. The module will also output the
correctly-received data byte. `out_byte` needs to be valid when `done` is 1, and is
don't-care otherwise (8'bx). If the stop bit does not appear when expected, the FSM
enters error state and must wait until it finds a stop bit before attempting to
receive the next byte. Include a active-high synchronous reset. Note that the serial
protocol `in` sends in a sequence from LSB to MSB. Assume all sequential logic
is triggered on the positive edge of the clock.
### Completed Verilog Module
```verilog
module TopModule (
   input  logic clk,
   input  logic in,
   input  logic reset,
   output logic [7:0] out_byte,
   output logic done
);
   // State definitions
   localparam IDLE = 3'b000;
   localparam RECEIVE = 3'b001;
   localparam CHECK_STOP = 3'b010;
   localparam ERROR = 3'b011;
   // State register
   logic [2:0] state;
   logic [2:0] next_state;
   // Data bit counter
   logic [3:0] bit_count;
   // Data storage
   logic [7:0] data_buffer;
   // FSM logic to handle state transitions and outputs
   always @(posedge clk) begin
      if (reset) begin
         state <= IDLE;
         bit_count <= 0;
         data_buffer <= 0;
         done <= 0;
      end else begin
         state <= next_state;
```

```
    end
  end
  // Combinational logic for next state and output control
  always @(*) begin
    next_state = state; // Default to stay in current state
    done = 0; // Default done to 0
    case (state)
      IDLE: begin
        if (in == 0) begin
          next_state = RECEIVE;
        end
      end
      RECEIVE: begin
        if (bit_count == 7) begin // Check if 8 bits have been received
          next_state = CHECK_STOP;
        end
      end
      CHECK_STOP: begin
        if (in == 1) begin
          next_state = IDLE;
          done = 1;
          out_byte = data_buffer;
        end else begin
          next_state = ERROR;
        end
      end
      ERROR: begin
        if (in == 1) begin
          next_state = IDLE;
        end
      end
    endcase
  end
  // Data reception logic
  always @(posedge clk) begin
    if (state == RECEIVE) begin
      data_buffer <= {in, data_buffer[7:1]}; // Shift register operation
      bit_count <= bit_count + 1;
    end else begin
      bit_count <= 0;
    end
  end
endmodule
```
[Instructions]:
1. Use the verilog_simulation_tool to verify the syntax and functional correctness of the Completed Verilog Module.
2. Use the waveform_trace_tool to trace the waveform and partial verilog code of functional incorrect signals.
3. Debug the waveform and verilog source code and find out the signals need to be corrected.
4. Repeat above steps until pass the syntax and functional check.

[Constraints]:
- Do not use typedef enum in the verilog code.
- There is test bench to test the functional correctness. You don't need to generate testbench to test the generated verilog code.
- Do not use $display or $finish in the module implementation.
- You can not modify the testbench.
- Declare all ports as logic; use wire or reg for signals inside the block.
- Don't use state_t. Use 'reg' or 'logic' for signals as registers or Flip-Flops.
- for combinational logic, you can use wire assign or always @(*).

- for combinational logic with an always block do not explicitly specify the sensitivity list; instead use always @(*)
- Don't generate duplicated signal assignments or blocks.
--------------------------------------------------------------------------------
**verilog_engineer (to chat_manager):**
***** Suggested tool call (call_ecH4qlKB5Hy8RR7nPhtw6wgZ): verilog_simulation_tool *****
Arguments:
{"completed_verilog":"module TopModule (\n    input  logic clk,\n    input  logic in,\n    input  logic reset,\n    output logic [7:0] out_byte,\n    output logic done\n);\n\n    // State definitions\n    localparam IDLE = 3'b000;\n    localparam RECEIVE = 3'b001;\n    localparam CHECK_STOP = 3'b010;\n    localparam ERROR = 3'b011;\n\n    // State register\n    logic [2:0] state;\n    logic [2:0] next_state;\n\n    // Data bit counter\n    logic [3:0] bit_count;\n\n    // Data storage\n    logic [7:0] data_buffer;\n\n    // FSM logic to handle state transitions and outputs\n    always @(posedge clk) begin\n        if (reset) begin\n            state <= IDLE;\n            bit_count <= 0;\n            data_buffer <= 0;\n            done <= 0;\n        end else begin\n            state <= next_state;\n        end\n    end\n\n    // Combinational logic for next state and output control\n    always @(*) begin\n        next_state = state; // Default to stay in current state\n        done = 0; // Default done to 0\n        case (state)\n            IDLE: begin\n                if (in == 0) begin\n                    next_state = RECEIVE;\n                end\n            end\n            RECEIVE: begin\n                if (bit_count == 7) begin // Check if 8 bits have been received\n                    next_state = CHECK_STOP;\n                end\n            end\n            CHECK_STOP: begin\n                if (in == 1) begin\n                    next_state = IDLE;\n                    done = 1;\n                    out_byte = data_buffer;\n                end else begin\n                    next_state = ERROR;\n                end\n            end\n            ERROR: begin\n                if (in == 1) begin\n                    next_state = IDLE;\n                end\n            end\n        endcase\n    end\n\n    // Data reception logic\n    always @(posedge clk) begin\n        if (state == RECEIVE) begin\n            data_buffer <= {in, data_buffer[7:1]}; // Shift register operation\n            bit_count <= bit_count + 1;\n        end else begin\n            bit_count <= 0;\n        end\n    end\n\nendmodule"}
***************************************************************************************
--------------------------------------------------------------------------------
>>>>>>>> EXECUTING FUNCTION verilog_simulation_tool...
user (to chat_manager):
user (to chat_manager):
***** Response from calling tool (call_ecH4qlKB5Hy8RR7nPhtw6wgZ) *****
[Compiled Success]
[Function Check Failed]
==Report start==
VCD info: dumpfile wave.vcd opened for output.
VCD warning: $dumpvars: Package ($unit) is not dumpable with VCD.
./test.sv:45: $finish called at 4526 (1ps)
Hint: Output 'out_byte' has no mismatches.
Hint: Output 'done' has 72 mismatches. First mismatch occurred at time 100.
Hint: Total mismatched samples is 72 out of 905 samples
Simulation finished at 4526 ps
Mismatches: 72 in 905 samples
==Report End==
Thought: input above output tool response into waveform_trace_tool to debug the failed signals starts with trace_level=2!
**********************************************************************
--------------------------------------------------------------------------------
**verilog_engineer (to chat_manager):**
***** Suggested tool call (call_lZFxSVZknlv7K9qKCiPPPph7): waveform_trace_tool *****
Arguments:
{"function_check_output":"[Compiled Success]\n[Function Check Failed]\n==Report start==\nVCD info: dumpfile wave.vcd opened for output.\nVCD warning: $dumpvars: Package ($unit) is not dumpable with VCD.\n./test.sv:45: $finish called at 4526 (1ps)\nHint: Output 'out_byte' has no mismatches.\nHint: Output 'done' has 72 mismatches. First mismatch occurred at time 100.\nHint: Total mismatched samples is 72 out of 905 samples\n\nSimulation finished at 4526 ps\nMismatches: 72 in 905 samples\n==Report End==","trace_level":2}
***********************************************************************************
--------------------------------------------------------------------------------
>>>>>>>> EXECUTING FUNCTION waveform_trace_tool...
Creating new AST tree graph...
Generating LALR tables
WARNING: 183 shift/reduce conflicts
Get mismatched signal...

Hint: Total mismatched samples is 72 out of 905 samples
mismatches = 72
Trace graph signal...
deque([('reset', 'done'), ('in', 'done'), ('state', 'done')])
deque([('state', 'in'), ('next_state', 'state')])
deque([('next_state', 'state'), ('bit_count', 'next_state')])
Get table waveform...
['done_ref', 'in_ref', 'reset_ref'] ['done_dut', 'in_dut', 'reset_dut'] ['done', 'clk', 'in', 'reset']
data frame shape = 5 20
user (to chat_manager):
user (to chat_manager):
***** Response from calling tool (call_lZFxSVZknlv7K9qKCiPPPph7) *****
[Verilog of DUT]:
```verilog
module TopModule (
  input  logic clk,
  input  logic in,
  input  logic reset,
  output logic [7:0] out_byte,
  output logic done
);
  // State definitions
  localparam IDLE = 3'b000;
  localparam RECEIVE = 3'b001;
  localparam CHECK_STOP = 3'b010;
  localparam ERROR = 3'b011;
  // State register
  logic [2:0] state;
  logic [2:0] next_state;
  // Data bit counter
  logic [3:0] bit_count;
  // Data storage
  logic [7:0] data_buffer;
  // FSM logic to handle state transitions and outputs
  always @(posedge clk) begin
    if (reset) begin
      state <= IDLE;
      bit_count <= 0;
      data_buffer <= 0;
      done <= 0;
    end else begin
      state <= next_state;
    end
  end
  // Combinational logic for next state and output control
  always @(*) begin
    next_state = state; // Default to stay in current state
    done = 0; // Default done to 0
    case (state)
      IDLE: begin
        if (in == 0) begin
          next_state = RECEIVE;
        end
      end
      RECEIVE: begin
        if (bit_count == 7) begin // Check if 8 bits have been received
          next_state = CHECK_STOP;
        end
```

```
      end
      CHECK_STOP: begin
        if (in == 1) begin
          next_state = IDLE;
          done = 1;
          out_byte = data_buffer;
        end else begin
          next_state = ERROR;
        end
      end
      ERROR: begin
        if (in == 1) begin
          next_state = IDLE;
        end
      end
    endcase
  end
  // Data reception logic
  always @(posedge clk) begin
    if (state == RECEIVE) begin
      data_buffer <= {in, data_buffer[7:1]}; // Shift register operation
      bit_count <= bit_count + 1;
    end else begin
      bit_count <= 0;
    end
  end
endmodule
```
[Siganl Waveform]: <signal>_tb is the given testbench signal and can not be changed! <signal>_ref is the golden, and <signal>_dut is the generated verilog file waveform. Check the mismatched signal waveform and its traced signals. The clock cycle (clk) is 10ns and toggles every 5ns.
'-' means unknown during simulation. If the '-' is the reason of mismatched signal, please check the reset and assignment block.
[Testbench Input Port Signal to Module]: clk, in, reset
[Traced Signals]: done, reset, in, state, next_state, clk
[Table Waveform in hexadecimal format]
### First mismatched signals time(ns) Trace ###

| time(ns) | done_dut | done_ref | in_dut | in_ref | next_state_dut[2:0] | reset_dut | reset_ref | state_dut[2:0] |
|---|---|---|---|---|---|---|---|---|
| 0 | 0 | - | 1 | 1 | - | 1 | 1 | - |
| 5 | 0 | 0 | 0 | 0 | 1 | 0 | 0 | 0 |
| 15 | 0 | 0 | 0 | 0 | 1 | 0 | 0 | 1 |
| 85 | 0 | 0 | 0 | 0 | 2 | 0 | 0 | 1 |
| 95 | 1 | 0 | 1 | 1 | 0 | 0 | 0 | 2 |

### First mismatched signals time(ns) End ###
The values of mismatched signals at the first mismatched signal time above:
done_dut: 1
done_ref: 0
in_dut: 1
in_ref: 1
reset_dut: 0
reset_ref: 0
### Mismatched signals time(ns) Trace After the First Mismatch ###

| time(ns) | done_dut | done_ref | in_dut | in_ref | next_state_dut[2:0] | reset_dut | reset_ref | state_dut[2:0] |
|---|---|---|---|---|---|---|---|---|
| 0 | 0 | - | 1 | 1 | - | 1 | 1 | - |
| 5 | 0 | 0 | 0 | 0 | 1 | 0 | 0 | 0 |
| 15 | 0 | 0 | 0 | 0 | 1 | 0 | 0 | 1 |

| | | | | | | | | |
|---|---|---|---|---|---|---|---|---|
| 85 | 0 | 0 | 0 | 0 | 2 | 0 | 0 | 1 |
| 95 | 1 | 0 | 1 | 1 | 0 | 0 | 0 | 2 |
| 105 | 0 | 1 | 0 | 0 | 1 | 0 | 0 | 0 |
| 110 | 0 | 1 | 0 | 0 | 1 | 0 | 0 | 0 |
| 115 | 0 | 0 | 0 | 0 | 1 | 0 | 0 | 1 |
| 120 | 0 | 0 | 0 | 0 | 1 | 0 | 0 | 1 |

### Mismatched signals time(ns) Trace After the First Mismatch End ###
[Note] You can not change the [testbench input signal]: (clk, in, reset)! Modify the module implementation considering the input signals.
[Hint] Firstly, identify the time of mismatched signals, and only focus on the mistmatched signals in the waveform firstly.Then, explain the related signals and their transitions in the waveform table. Don't correct signals without mismatch in the table waveforms.If the information is not enough for correct the functional error, try to trace more relevant signals using trace_level >2 for waveform_trace_tool.If you know how to correct the functional error, start to correct the code and run verilog_simulation_tool again.
**********************************************************************
--------------------------------------------------------------------------------
Removed 1 messages. Number of messages reduced from 5 to 4.
**verilog_engineer (to chat_manager):**
The waveform trace indicates that the `done` signal is set incorrectly at time 95 ns when it should remain 0. The issue occurs because the `done` signal is set to 1 in the `CHECK_STOP` state without ensuring that all 8 bits have been correctly received and the stop bit is verified.
In the current implementation, the transition from `RECEIVE` to `CHECK_STOP` occurs when `bit_count` equals 7, which is incorrect because the bit count should reach 8 to ensure all bits are received. The `bit_count` should be checked against 8 instead of 7 before transitioning to `CHECK_STOP`.
Let's correct the code by adjusting the condition for transitioning from `RECEIVE` to `CHECK_STOP` and ensure that `done` is set correctly based on the complete reception of the byte and the correct stop bit.
### Corrected Verilog Module
```verilog
module TopModule (
  input  logic clk,
  input  logic in,
  input  logic reset,
  output logic [7:0] out_byte,
  output logic done
);
  // State definitions
  localparam IDLE = 3'b000;
  localparam RECEIVE = 3'b001;
  localparam CHECK_STOP = 3'b010;
  localparam ERROR = 3'b011;
  // State register
  logic [2:0] state;
  logic [2:0] next_state;
  // Data bit counter
  logic [3:0] bit_count;
  // Data storage
  logic [7:0] data_buffer;
  // FSM logic to handle state transitions and outputs
  always @(posedge clk) begin
    if (reset) begin
      state <= IDLE;
      bit_count <= 0;
      data_buffer <= 0;
      done <= 0;
    end else begin
      state <= next_state;
    end
  end
```

```
  // Combinational logic for next state and output control
  always @(*) begin
    next_state = state; // Default to stay in current state
    done = 0; // Default done to 0
    case (state)
      IDLE: begin
        if (in == 0) begin
          next_state = RECEIVE;
        end
      end
      RECEIVE: begin
        if (bit_count == 8) begin // Check if 8 bits have been received
          next_state = CHECK_STOP;
        end
      end
      CHECK_STOP: begin
        if (in == 1) begin
          next_state = IDLE;
          done = 1;
          out_byte = data_buffer;
        end else begin
          next_state = ERROR;
        end
      end
      ERROR: begin
        if (in == 1) begin
          next_state = IDLE;
        end
      end
    endcase
  end
  // Data reception logic
  always @(posedge clk) begin
    if (state == RECEIVE) begin
      data_buffer <= {in, data_buffer[7:1]}; // Shift register operation
      bit_count <= bit_count + 1;
    end else begin
      bit_count <= 0;
    end
  end
endmodule
```

Now, let's re-run the simulation tool to verify the corrected module.
***** Suggested tool call (call_lZFxSVZknlv7K9qKCiPPPph7): verilog_simulation_tool *****
Arguments:
{"completed_verilog":"module TopModule (\n input logic clk,\n input logic in,\n input logic reset,\n output logic [7:0] out_byte,\n output logic done\n);\n\n // State definitions\n localparam IDLE = 3'b000;\n localparam RECEIVE = 3'b001;\n localparam CHECK_STOP = 3'b010;\n localparam ERROR = 3'b011;\n\n // State register\n logic [2:0] state;\n logic [2:0] next_state;\n\n // Data bit counter\n logic [3:0] bit_count;\n\n // Data storage\n logic [7:0] data_buffer;\n\n // FSM logic to handle state transitions and outputs\n always @(posedge clk) begin\n if (reset) begin\n state <= IDLE;\n bit_count <= 0;\n data_buffer <= 0;\n done <= 0;\n end else begin\n state <= next_state;\n end\n end\n\n // Combinational logic for next state and output control\n always @(*) begin\n next_state = state; // Default to stay in current state\n done = 0; // Default done to 0\n case (state)\n IDLE: begin\n if (in == 0) begin\n next_state = RECEIVE;\n end\n end\n RECEIVE: begin\n if (bit_count == 8) begin // Check if 8 bits have been received\n next_state = CHECK_STOP;\n end\n end\n CHECK_STOP: begin\n if (in == 1) begin\n next_state = IDLE;\n done = 1;\n out_byte = data_buffer;\n end else begin\n next_state = ERROR;\n end\n end\n ERROR: begin\n if (in == 1) begin\n next_state = IDLE;\n end\n end\n endcase\n end\n\n // Data

reception logic\n    always @(posedge clk) begin\n        if (state == RECEIVE) begin\n            data_buffer <= {in, data_buffer[7:1]}; // Shift register operation\n            bit_count <= bit_count + 1;\n        end else begin\n            bit_count <= 0;\n        end\n    end\n\nendmodule"}
******************************************************************************************
--------------------------------------------------------------------------------
>>>>>>>> EXECUTING FUNCTION verilog_simulation_tool...
user (to chat_manager):
user (to chat_manager):
***** Response from calling tool (call_lZFxSVZknlv7K9qKCiPPPph7) *****
[Compiled Success]
[Function Check Failed]
==Report start==
VCD info: dumpfile wave.vcd opened for output.
VCD warning: $dumpvars: Package ($unit) is not dumpable with VCD.
./test.sv:45: $finish called at 4526 (1ps)
Hint: Output 'out_byte' has 38 mismatches. First mismatch occurred at time 110.
Hint: Output 'done' has 47 mismatches. First mismatch occurred at time 110.
Hint: Total mismatched samples is 57 out of 905 samples
Simulation finished at 4526 ps
Mismatches: 57 in 905 samples
==Report End==
Thought: input above output tool response into waveform_trace_tool to debug the failed signals starts with trace_level=2!
**********************************************************************
--------------------------------------------------------------------------------
Removed 3 messages. Number of messages reduced from 7 to 4.
**verilog_engineer (to chat_manager):**
***** Suggested tool call (call_MYioyiyi7N5onObBsxGM5Whb): waveform_trace_tool *****
Arguments:
{"function_check_output":"[Compiled Success]\n[Function Check Failed]\n==Report start==\nVCD info: dumpfile wave.vcd opened for output.\nVCD warning: $dumpvars: Package ($unit) is not dumpable with VCD.\n./test.sv:45: $finish called at 4526 (1ps)\nHint: Output 'out_byte' has 38 mismatches. First mismatch occurred at time 110.\nHint: Output 'done' has 47 mismatches. First mismatch occurred at time 110.\nHint: Total mismatched samples is 57 out of 905 samples\n\nSimulation finished at 4526 ps\nMismatches: 57 in 905 samples\n==Report End==","trace_level":2}
**************************************************************************************
--------------------------------------------------------------------------------
>>>>>>>> EXECUTING FUNCTION waveform_trace_tool...
Creating new AST tree graph...
Generating LALR tables
WARNING: 183 shift/reduce conflicts
Get mismatched signal...
Hint: Total mismatched samples is 57 out of 905 samples
mismatches =  57
Trace graph signal...
deque([('data_buffer', 'out_byte'), ('in', 'out_byte'), ('state', 'out_byte'), ('reset', 'done'), ('in', 'done'), ('state', 'done')])
deque([('reset', 'data_buffer'), ('in', 'data_buffer'), ('state', 'data_buffer'), ('state', 'in'), ('next_state', 'state'), ('reset', 'state'), ('next_state', 'state')])
deque([('next_state', 'state'), ('next_state', 'state'), ('bit_count', 'next_state'), ('bit_count', 'next_state')])
Get table waveform...
['done_ref', 'in_ref', 'out_byte_ref[7:0]', 'reset_ref'] ['done_dut', 'in_dut', 'out_byte_dut[7:0]', 'reset_dut'] ['out_byte', 'done', 'clk', 'in', 'reset']
Failed to transform to binary  out_byte_dut[7:0]  target line:  -
data frame shape =  5   20
user (to chat_manager):
user (to chat_manager):
***** Response from calling tool (call_MYioyiyi7N5onObBsxGM5Whb) *****
[Verilog of DUT]:
```verilog
module TopModule (
```

```
    input  logic clk,
    input  logic in,
    input  logic reset,
    output logic [7:0] out_byte,
    output logic done
);
    // State definitions
    localparam IDLE = 3'b000;
    localparam RECEIVE = 3'b001;
    localparam CHECK_STOP = 3'b010;
    localparam ERROR = 3'b011;
    // State register
    logic [2:0] state;
    logic [2:0] next_state;
    // Data bit counter
    logic [3:0] bit_count;
    // Data storage
    logic [7:0] data_buffer;
    // FSM logic to handle state transitions and outputs
    always @(posedge clk) begin
        if (reset) begin
            state <= IDLE;
            bit_count <= 0;
            data_buffer <= 0;
            done <= 0;
        end else begin
            state <= next_state;
        end
    end
    // Combinational logic for next state and output control
    always @(*) begin
        next_state = state; // Default to stay in current state
        done = 0; // Default done to 0
        case (state)
            IDLE: begin
                if (in == 0) begin
                    next_state = RECEIVE;
                end
            end
            RECEIVE: begin
                if (bit_count == 8) begin // Check if 8 bits have been received
                    next_state = CHECK_STOP;
                end
            end
            CHECK_STOP: begin
                if (in == 1) begin
                    next_state = IDLE;
                    done = 1;
                    out_byte = data_buffer;
                end else begin
                    next_state = ERROR;
                end
            end
            ERROR: begin
                if (in == 1) begin
                    next_state = IDLE;
                end
            end
```

```
      endcase
    end
    // Data reception logic
    always @(posedge clk) begin
      if (state == RECEIVE) begin
        data_buffer <= {in, data_buffer[7:1]}; // Shift register operation
        bit_count <= bit_count + 1;
      end else begin
        bit_count <= 0;
      end
    end
endmodule
```

[Siganl Waveform]: <signal>_tb is the given testbench signal and can not be changed! <signal>_ref is the golden, and <signal>_dut is the generated verilog file waveform. Check the mismatched signal waveform and its traced signals. The clock cycle (clk) is 10ns and toggles every 5ns.
'-' means unknown during simulation. If the '-' is the reason of mismatched signal, please check the reset and assignment block.
[Testbench Input Port Signal to Module]: clk, in, reset
[Traced Signals]: out_byte, done, data_buffer, in, state, reset, next_state, clk
[Table Waveform in hexadecimal format]
### First mismatched signals time(ns) Trace ###

| time(ns) | data_buffer_dut[7:0] | done_dut | done_ref | in_dut | in_ref | next_state_dut[2:0] | out_byte_dut[7:0] | out_byte_ref[7:0] | reset_dut | reset_ref | state_dut[2:0] |
|---|---|---|---|---|---|---|---|---|---|---|---|
| 0 | - | 0 | - | 1 | 1 | - | - | - | 1 | 1 | - |
| 5 | 0 | 0 | 0 | 0 | 0 | 1 | - | - | 0 | 0 | 0 |
| 15 | 0 | 0 | 0 | 0 | 0 | 1 | - | - | 0 | 0 | 1 |
| 95 | 0 | 0 | 0 | 1 | 1 | 2 | - | - | 0 | 0 | 1 |
| 105 | 80 | 0 | 1 | 0 | 0 | 3 | - | 0 | 0 | 0 | 2 |

### First mismatched signals time(ns) End ###
The values of mismatched signals at the first mismatched signal time above:
done_dut: 0
done_ref: 1
in_dut: 0
in_ref: 0
out_byte_dut[7:0]: -
out_byte_ref[7:0]: 0000
reset_dut: 0
reset_ref: 0
### Mismatched signals time(ns) Trace After the First Mismatch ###

| time(ns) | data_buffer_dut[7:0] | done_dut | done_ref | in_dut | in_ref | next_state_dut[2:0] | out_byte_dut[7:0] | out_byte_ref[7:0] | reset_dut | reset_ref | state_dut[2:0] |
|---|---|---|---|---|---|---|---|---|---|---|---|
| 0 | - | 0 | - | 1 | 1 | - | - | - | 1 | 1 | - |
| 5 | 0 | 0 | 0 | 0 | 0 | 1 | - | - | 0 | 0 | 0 |
| 15 | 0 | 0 | 0 | 0 | 0 | 1 | - | - | 0 | 0 | 1 |
| 95 | 0 | 0 | 0 | 1 | 1 | 2 | - | - | 0 | 0 | 1 |
| 105 | 80 | 0 | 1 | 0 | 0 | 3 | - | 0 | 0 | 0 | 2 |
| 115 | 80 | 0 | 0 | 0 | 0 | 3 | - | - | 0 | 0 | 3 |
| 120 | 80 | 0 | 0 | 0 | 0 | 3 | - | - | 0 | 0 | 3 |
| 125 | 80 | 0 | 0 | 0 | 0 | 3 | - | - | 0 | 0 | 3 |
| 130 | 80 | 0 | 0 | 0 | 0 | 3 | - | - | 0 | 0 | 3 |

### Mismatched signals time(ns) Trace After the First Mismatch End ###
[Note] You can not change the [testbench input signal]: (clk, in, reset)! Modify the module implementation considering the input signals.
[Hint] Firstly, identify the time of mismatched signals, and only focus on the mistmatched signals in the waveform firstly.Then, explain the related signals and their transitions in the waveform table. Don't correct signals without mismatch

in the table waveforms.If the information is not enough for correct the functional error, try to trace more relevant signals using trace_level >2 for waveform_trace_tool.If you know how to correct the functional error, start to correct the code and run verilog_simulation_tool again.
**********************************************************************
--------------------------------------------------------------------------------
Removed 5 messages. Number of messages reduced from 9 to 4.
**verilog_engineer (to chat_manager):**
The waveform trace indicates that the `done` signal is set incorrectly at time 105 ns when it should be 1, but it remains 0. This issue arises because the transition from the `RECEIVE` state to the `CHECK_STOP` state is based on the `bit_count` reaching 8, but the `bit_count` is incremented after the data is shifted into `data_buffer`. This results in the `CHECK_STOP` state being entered one clock cycle too late, causing the `done` signal to be set incorrectly.
To fix this, we need to adjust the condition for incrementing the `bit_count` and transitioning to the `CHECK_STOP` state. The `bit_count` should be incremented before checking if it has reached 8, and the transition to `CHECK_STOP` should occur when `bit_count` equals 7 (since it will be incremented to 8 in the same cycle).
### Corrected Verilog Module
```verilog
module TopModule (
  input  logic clk,
  input  logic in,
  input  logic reset,
  output logic [7:0] out_byte,
  output logic done
);
  // State definitions
  localparam IDLE = 3'b000;
  localparam RECEIVE = 3'b001;
  localparam CHECK_STOP = 3'b010;
  localparam ERROR = 3'b011;
  // State register
  logic [2:0] state;
  logic [2:0] next_state;
  // Data bit counter
  logic [3:0] bit_count;
  // Data storage
  logic [7:0] data_buffer;
  // FSM logic to handle state transitions and outputs
  always @(posedge clk) begin
    if (reset) begin
      state <= IDLE;
      bit_count <= 0;
      data_buffer <= 0;
      done <= 0;
    end else begin
      state <= next_state;
    end
  end
  // Combinational logic for next state and output control
  always @(*) begin
    next_state = state; // Default to stay in current state
    done = 0; // Default done to 0
    case (state)
      IDLE: begin
        if (in == 0) begin
          next_state = RECEIVE;
        end
      end
      RECEIVE: begin
        if (bit_count == 7) begin // Check if 8 bits have been received
```

```
          next_state = CHECK_STOP;
        end
      end
      CHECK_STOP: begin
        if (in == 1) begin
          next_state = IDLE;
          done = 1;
          out_byte = data_buffer;
        end else begin
          next_state = ERROR;
        end
      end
      ERROR: begin
        if (in == 1) begin
          next_state = IDLE;
        end
      end
    endcase
  end
  // Data reception logic
  always @(posedge clk) begin
    if (state == RECEIVE) begin
      bit_count <= bit_count + 1;
      data_buffer <= {in, data_buffer[7:1]}; // Shift register operation
    end else begin
      bit_count <= 0;
    end
  end
endmodule
```

Now, let's re-run the simulation tool to verify the corrected module.
***** Suggested tool call (call_WgxSQT2R7NjyLQtvREVvaxAj): verilog_simulation_tool *****
Arguments:
{"completed_verilog":"module TopModule (\n input logic clk,\n input logic in,\n input logic reset,\n output logic [7:0] out_byte,\n output logic done\n);\n\n // State definitions\n localparam IDLE = 3'b000;\n localparam RECEIVE = 3'b001;\n localparam CHECK_STOP = 3'b010;\n localparam ERROR = 3'b011;\n\n // State register\n logic [2:0] state;\n logic [2:0] next_state;\n\n // Data bit counter\n logic [3:0] bit_count;\n\n // Data storage\n logic [7:0] data_buffer;\n\n // FSM logic to handle state transitions and outputs\n always @(posedge clk) begin\n if (reset) begin\n state <= IDLE;\n bit_count <= 0;\n data_buffer <= 0;\n done <= 0;\n end else begin\n state <= next_state;\n end\n end\n\n // Combinational logic for next state and output control\n always @(*) begin\n next_state = state; // Default to stay in current state\n done = 0; // Default done to 0\n case (state)\n IDLE: begin\n if (in == 0) begin\n next_state = RECEIVE;\n end\n end\n RECEIVE: begin\n if (bit_count == 7) begin // Check if 8 bits have been received\n next_state = CHECK_STOP;\n end\n end\n CHECK_STOP: begin\n if (in == 1) begin\n next_state = IDLE;\n done = 1;\n out_byte = data_buffer;\n end else begin\n next_state = ERROR;\n end\n end\n ERROR: begin\n if (in == 1) begin\n next_state = IDLE;\n end\n end\n endcase\n end\n\n // Data reception logic\n always @(posedge clk) begin\n if (state == RECEIVE) begin\n bit_count <= bit_count + 1;\n data_buffer <= {in, data_buffer[7:1]}; // Shift register operation\n end else begin\n bit_count <= 0;\n end\n end\n\nendmodule"}
*************************************************************************************
--------------------------------------------------------------------------------
>>>>>>>> EXECUTING FUNCTION verilog_simulation_tool...
user (to chat_manager):
user (to chat_manager):
***** Response from calling tool (call_WgxSQT2R7NjyLQtvREVvaxAj) *****
[Compiled Success]
[Function Check Failed]
==Report start==

VCD info: dumpfile wave.vcd opened for output.
VCD warning: $dumpvars: Package ($unit) is not dumpable with VCD.
./test.sv:45: $finish called at 4526 (1ps)
Hint: Output 'out_byte' has no mismatches.
Hint: Output 'done' has 72 mismatches. First mismatch occurred at time 100.
Hint: Total mismatched samples is 72 out of 905 samples
Simulation finished at 4526 ps
Mismatches: 72 in 905 samples
==Report End==
Thought: input above output tool response into waveform_trace_tool to debug the failed signals starts with trace_level=2!
**********************************************************************
--------------------------------------------------------------------------------
Removed 7 messages. Number of messages reduced from 11 to 4.
**verilog_engineer (to chat_manager):**
***** Suggested tool call (call_e9LsUJLEQx1HvJpMaQtYPnAm): waveform_trace_tool *****
Arguments:
{"function_check_output":"[Compiled Success]\n[Function Check Failed]\n==Report start==\nVCD info: dumpfile wave.vcd opened for output.\nVCD warning: $dumpvars: Package ($unit) is not dumpable with VCD.\n./test.sv:45: $finish called at 4526 (1ps)\nHint: Output 'out_byte' has no mismatches.\nHint: Output 'done' has 72 mismatches. First mismatch occurred at time 100.\nHint: Total mismatched samples is 72 out of 905 samples\n\nSimulation finished at 4526 ps\nMismatches: 72 in 905 samples\n==Report End==","trace_level":2}
**************************************************************************************
--------------------------------------------------------------------------------
>>>>>>>> EXECUTING FUNCTION waveform_trace_tool...
Creating new AST tree graph...
Generating LALR tables
WARNING: 183 shift/reduce conflicts
Get mismatched signal...
Hint: Total mismatched samples is 72 out of 905 samples
mismatches =  72
Trace graph signal...
deque([('reset', 'done'), ('in', 'done'), ('state', 'done')])
deque([('state', 'in'), ('next_state', 'state')])
deque([('next_state', 'state'), ('bit_count', 'next_state')])
Get table waveform...
['done_ref', 'in_ref', 'reset_ref'] ['done_dut', 'in_dut', 'reset_dut'] ['done', 'clk', 'in', 'reset']
data frame shape =  5   20
user (to chat_manager):
user (to chat_manager):
***** Response from calling tool (call_e9LsUJLEQx1HvJpMaQtYPnAm) *****
[Verilog of DUT]:
```verilog
module TopModule (
   input  logic clk,
   input  logic in,
   input  logic reset,
   output logic [7:0] out_byte,
   output logic done
);
   // State definitions
   localparam IDLE = 3'b000;
   localparam RECEIVE = 3'b001;
   localparam CHECK_STOP = 3'b010;
   localparam ERROR = 3'b011;
   // State register
   logic [2:0] state;
   logic [2:0] next_state;
   // Data bit counter
```

```
  logic [3:0] bit_count;
  // Data storage
  logic [7:0] data_buffer;
  // FSM logic to handle state transitions and outputs
  always @(posedge clk) begin
    if (reset) begin
      state <= IDLE;
      bit_count <= 0;
      data_buffer <= 0;
      done <= 0;
    end else begin
      state <= next_state;
    end
  end
  // Combinational logic for next state and output control
  always @(*) begin
    next_state = state; // Default to stay in current state
    done = 0; // Default done to 0
    case (state)
      IDLE: begin
        if (in == 0) begin
          next_state = RECEIVE;
        end
      end
      RECEIVE: begin
        if (bit_count == 7) begin // Check if 8 bits have been received
          next_state = CHECK_STOP;
        end
      end
      CHECK_STOP: begin
        if (in == 1) begin
          next_state = IDLE;
          done = 1;
          out_byte = data_buffer;
        end else begin
          next_state = ERROR;
        end
      end
      ERROR: begin
        if (in == 1) begin
          next_state = IDLE;
        end
      end
    endcase
  end
  // Data reception logic
  always @(posedge clk) begin
    if (state == RECEIVE) begin
      bit_count <= bit_count + 1;
      data_buffer <= {in, data_buffer[7:1]}; // Shift register operation
    end else begin
      bit_count <= 0;
    end
  end
endmodule
```

[Siganl Waveform]: <signal>_tb is the given testbench signal and can not be changed! <signal>_ref is the golden, and <signal>_dut is the generated verilog file waveform. Check the mismatched signal waveform and its traced signals. The clock cycle (clk) is 10ns and toggles every 5ns.
'-' means unknown during simulation. If the '-' is the reason of mismatched signal, please check the reset and assignment block.
[Testbench Input Port Signal to Module]: clk, in, reset
[Traced Signals]: done, reset, in, state, next_state, clk
[Table Waveform in hexadecimal format]
### First mismatched signals time(ns) Trace ###

| time(ns) | done_dut | done_ref | in_dut | in_ref | next_state_dut[2:0] | reset_dut | reset_ref | state_dut[2:0] |
|---|---|---|---|---|---|---|---|---|
| 0 | 0 | - | 1 | 1 | - | 1 | 1 | - |
| 5 | 0 | 0 | 0 | 0 | 1 | 0 | 0 | 0 |
| 15 | 0 | 0 | 0 | 0 | 1 | 0 | 0 | 1 |
| 85 | 0 | 0 | 0 | 0 | 2 | 0 | 0 | 1 |
| 95 | 1 | 0 | 1 | 1 | 0 | 0 | 0 | 2 |

### First mismatched signals time(ns) End ###
The values of mismatched signals at the first mismatched signal time above:
done_dut: 1
done_ref: 0
in_dut: 1
in_ref: 1
reset_dut: 0
reset_ref: 0
### Mismatched signals time(ns) Trace After the First Mismatch ###

| time(ns) | done_dut | done_ref | in_dut | in_ref | next_state_dut[2:0] | reset_dut | reset_ref | state_dut[2:0] |
|---|---|---|---|---|---|---|---|---|
| 0 | 0 | - | 1 | 1 | - | 1 | 1 | - |
| 5 | 0 | 0 | 0 | 0 | 1 | 0 | 0 | 0 |
| 15 | 0 | 0 | 0 | 0 | 1 | 0 | 0 | 1 |
| 85 | 0 | 0 | 0 | 0 | 2 | 0 | 0 | 1 |
| 95 | 1 | 0 | 1 | 1 | 0 | 0 | 0 | 2 |
| 105 | 0 | 1 | 0 | 0 | 1 | 0 | 0 | 0 |
| 110 | 0 | 1 | 0 | 0 | 1 | 0 | 0 | 0 |
| 115 | 0 | 0 | 0 | 0 | 1 | 0 | 0 | 1 |
| 120 | 0 | 0 | 0 | 0 | 1 | 0 | 0 | 1 |

### Mismatched signals time(ns) Trace After the First Mismatch End ###
[Note] You can not change the [testbench input signal]: (clk, in, reset)! Modify the module implementation considering the input signals.
[Hint] Firstly, identify the time of mismatched signals, and only focus on the mistmatched signals in the waveform firstly.Then, explain the related signals and their transitions in the waveform table. Don't correct signals without mismatch in the table waveforms.If the information is not enough for correct the functional error, try to trace more relevant signals using trace_level >2 for waveform_trace_tool.If you know how to correct the functional error, start to correct the code and run verilog_simulation_tool again.
***********************************************************************
--------------------------------------------------------------------------------
Removed 9 messages. Number of messages reduced from 13 to 4.
**verilog_engineer (to chat_manager):**
The waveform trace reveals that the `done` signal is set incorrectly at 95 ns when it should be 0, but it is 1. This error occurs because the `done` signal is set to 1 in the `CHECK_STOP` state when `in` is 1, but it does not account for the transition back to the `IDLE` state before setting `done` back to 0.
To correct this, we need to ensure that the `done` signal is only set to 1 for one clock cycle when the stop bit is correctly received and then reset to 0 in the next clock cycle as the FSM transitions back to the `IDLE` state.
### Corrected Verilog Module
```verilog
module TopModule (
   input  logic clk,
   input  logic in,
```

```
    input  logic reset,
    output logic [7:0] out_byte,
    output logic done
);
    // State definitions
    localparam IDLE = 3'b000;
    localparam RECEIVE = 3'b001;
    localparam CHECK_STOP = 3'b010;
    localparam ERROR = 3'b011;
    // State register
    logic [2:0] state;
    logic [2:0] next_state;
    // Data bit counter
    logic [3:0] bit_count;
    // Data storage
    logic [7:0] data_buffer;
    // FSM logic to handle state transitions and outputs
    always @(posedge clk) begin
        if (reset) begin
            state <= IDLE;
            bit_count <= 0;
            data_buffer <= 0;
            done <= 0;
        end else begin
            state <= next_state;
            if (state == CHECK_STOP && in == 1) begin
                done <= 1; // Set done only for one cycle when stop bit is correct
            end else begin
                done <= 0;
            end
        end
    end
    // Combinational logic for next state and output control
    always @(*) begin
        next_state = state; // Default to stay in current state
        case (state)
            IDLE: begin
                if (in == 0) begin
                    next_state = RECEIVE;
                end
            end
            RECEIVE: begin
                if (bit_count == 7) begin // Check if 8 bits have been received
                    next_state = CHECK_STOP;
                end
            end
            CHECK_STOP: begin
                if (in == 1) begin
                    next_state = IDLE;
                    out_byte = data_buffer;
                end else begin
                    next_state = ERROR;
                end
            end
            ERROR: begin
                if (in == 1) begin
                    next_state = IDLE;
                end
```

```
        end
      endcase
    end
    // Data reception logic
    always @(posedge clk) begin
      if (state == RECEIVE) begin
        bit_count <= bit_count + 1;
        data_buffer <= {in, data_buffer[7:1]}; // Shift register operation
      end else begin
        bit_count <= 0;
      end
    end
endmodule
```

Now, let's re-run the simulation tool to verify the corrected module.
***** Suggested tool call (call_azcbF1Igu934nD80wolnesYr): verilog_simulation_tool *****
Arguments:
{"completed_verilog":"module TopModule (\n    input  logic clk,\n    input  logic in,\n    input  logic reset,\n    output logic [7:0] out_byte,\n    output logic done\n);\n\n    // State definitions\n    localparam IDLE = 3'b000;\n    localparam RECEIVE = 3'b001;\n    localparam CHECK_STOP = 3'b010;\n    localparam ERROR = 3'b011;\n\n    // State register\n    logic [2:0] state;\n    logic [2:0] next_state;\n\n    // Data bit counter\n    logic [3:0] bit_count;\n\n    // Data storage\n    logic [7:0] data_buffer;\n\n    // FSM logic to handle state transitions and outputs\n    always @(posedge clk) begin\n        if (reset) begin\n            state <= IDLE;\n            bit_count <= 0;\n            data_buffer <= 0;\n            done <= 0;\n        end else begin\n            state <= next_state;\n            if (state == CHECK_STOP && in == 1) begin\n                done <= 1; // Set done only for one cycle when stop bit is correct\n            end else begin\n                done <= 0;\n            end\n        end\n    end\n\n    // Combinational logic for next state and output control\n    always @(*) begin\n        next_state = state; // Default to stay in current state\n        case (state)\n            IDLE: begin\n                if (in == 0) begin\n                    next_state = RECEIVE;\n                end\n            end\n            RECEIVE: begin\n                if (bit_count == 7) begin // Check if 8 bits have been received\n                    next_state = CHECK_STOP;\n                end\n            end\n            CHECK_STOP: begin\n                if (in == 1) begin\n                    next_state = IDLE;\n                    out_byte = data_buffer;\n                end else begin\n                    next_state = ERROR;\n                end\n            end\n            ERROR: begin\n                if (in == 1) begin\n                    next_state = IDLE;\n                end\n            end\n        endcase\n    end\n\n    // Data reception logic\n    always @(posedge clk) begin\n        if (state == RECEIVE) begin\n            bit_count <= bit_count + 1;\n            data_buffer <= {in, data_buffer[7:1]}; // Shift register operation\n        end else begin\n            bit_count <= 0;\n        end\n    end\n\nendmodule"}
****************************************************************************************

--------------------------------------------------------------------------------

>>>>>>>> EXECUTING FUNCTION verilog_simulation_tool...
user (to chat_manager):
user (to chat_manager):
***** Response from calling tool (call_azcbF1Igu934nD80wolnesYr) *****
[Compiled Success]
[Function Check Success]
VCD info: dumpfile wave.vcd opened for output.
VCD warning: $dumpvars: Package ($unit) is not dumpable with VCD.
./test.sv:45: $finish called at 4526 (1ps)
Hint: Output 'out_byte' has no mismatches.
Hint: Output 'done' has no mismatches.
Hint: Total mismatched samples is 0 out of 905 samples
Simulation finished at 4526 ps
Mismatches: 0 in 905 samples
**********************************************************************

--------------------------------------------------------------------------------

Removed 11 messages. Number of messages reduced from 15 to 4.
**verilog_engineer (to chat_manager):**
TERMINATE

--------------------------------------------------------------------------------
