# Supplementary material for: VerilogCoder: Autonomous Verilog Coding Agents with Graph-based Planning and Abstract Syntax Tree (AST)-based Waveform Tracing Tool
Source: arXiv:2408.08927 source file (2025-03-05)
Supplement: Supplementary file 2 [file Appendix_debuglog.pdf]

**user (to chat\_manager):**

You are a Verilog RTL designer that only writes code using correct Verilog syntax and verify the functionality.

[Target Module Description]

### Problem

I would like you to implement a module named TopModule with the following interface. All input and output ports are one bit unless otherwise specified.

- input clk
- input in
- input reset
- output out\_byte (8 bits)
- output done

In many (older) serial communications protocols, each data byte is sent along with a start bit and a stop bit, to help the receiver delimit bytes from the stream of bits. One common scheme is to use one start bit (0), 8 data bits, and 1 stop bit (1). The `in` stays at logic 1 when nothing is being transmitted. The FSM should start to receive the following 8 data bits right after detect the start bit (0). Design a finite state machine that will identify when bytes have been correctly received when given a stream of bits. It needs to start to receive the data right away when the start bit (0) occurs, receive the consecutive all 8 data bits, then verify that the stop bit (1) was correct of `in`. `done` is set to 1 after verify the stop bit (1), otherwise, it will be remain 0. The module will also output the correctly-received data byte. `out\_byte` needs to be valid when `done` is 1, and is don't-care otherwise (8'bx). If the stop bit does not appear when expected, the FSM enters error state and must wait until it finds a stop bit before attempting to receive the next byte. Include a active-high synchronous reset. Note that the serial protocol `in` sends in a sequence from LSB to MSB. Assume all sequential logic is triggered on the positive edge of the clock.

### Completed Verilog Module

```
````verilog
module TopModule (
    input logic clk,
    input logic in,
    input logic reset,
    output logic [7:0] out_byte,
    output logic done
);
    // State definitions
    localparam IDLE = 3'b000;
    localparam RECEIVE = 3'b001;
    localparam CHECK_STOP = 3'b010;
    localparam ERROR = 3'b011;
    // State register
    logic [2:0] state;
    logic [2:0] next_state;
    // Data bit counter
    logic [3:0] bit_count;
    // Data storage
    logic [7:0] data_buffer;
    // FSM logic to handle state transitions and outputs
    always @(posedge clk) begin
        if (reset) begin
            state <= IDLE;
            bit_count <= 0;
            data_buffer <= 0;
            done <= 0;
        end else begin
            state <= next_state;
```

```

    end
end
// Combinational logic for next state and output control
always @(*) begin
    next_state = state; // Default to stay in current state
    done = 0; // Default done to 0
    case (state)
        IDLE: begin
            if (in == 0) begin
                next_state = RECEIVE;
            end
        end
        RECEIVE: begin
            if (bit_count == 7) begin // Check if 8 bits have been received
                next_state = CHECK_STOP;
            end
        end
        CHECK_STOP: begin
            if (in == 1) begin
                next_state = IDLE;
                done = 1;
                out_byte = data_buffer;
            end else begin
                next_state = ERROR;
            end
        end
        ERROR: begin
            if (in == 1) begin
                next_state = IDLE;
            end
        end
    endcase
end
// Data reception logic
always @(posedge clk) begin
    if (state == RECEIVE) begin
        data_buffer <= {in, data_buffer[7:1]}; // Shift register operation
        bit_count <= bit_count + 1;
    end else begin
        bit_count <= 0;
    end
end
endmodule
` ` `

```

[Instructions]:

1. Use the verilog\_simulation\_tool to verify the syntax and functional correctness of the Completed Verilog Module.
2. Use the waveform\_trace\_tool to trace the waveform and partial verilog code of functional incorrect signals.
3. Debug the waveform and verilog source code and find out the signals need to be corrected.
4. Repeat above steps until pass the syntax and functional check.

[Constraints]:

- Do not use typedef enum in the verilog code.
- There is test bench to test the functional correctness. You don't need to generate testbench to test the generated verilog code.
- Do not use \$display or \$finish in the module implementation.
- You can not modify the testbench.
- Declare all ports as logic; use wire or reg for signals inside the block.
- Don't use state\_t. Use 'reg' or 'logic' for signals as registers or Flip-Flops.
- for combinational logic, you can use wire assign or always @(\*).

- for combinational logic with an always block do not explicitly specify the sensitivity list; instead use always @(\*)
- Don't generate duplicated signal assignments or blocks.

#### verilog\_engineer (to chat\_manager):

\*\*\*\*\* Suggested tool call (call\_ecH4qKB5Hy8RR7nPhtw6wgZ): verilog\_simulation\_tool \*\*\*\*\*

Arguments:

```
{"completed_verilog": "module TopModule (\n  input logic clk,\n  input logic in,\n  input logic reset,\n  output logic [7:0] out_byte,\n  output logic done);\n\n  // State definitions\n  localparam IDLE = 3'b000;\n  localparam RECEIVE = 3'b001;\n  localparam CHECK_STOP = 3'b010;\n  localparam ERROR = 3'b011;\n\n  // State register\n  logic [2:0] state;\n  logic [2:0] next_state;\n\n  // Data bit counter\n  logic [3:0] bit_count;\n\n  // Data storage\n  logic [7:0] data_buffer;\n\n  // FSM logic to handle state transitions and outputs\n  always @(posedge clk) begin\n    if (reset) begin\n      state <= IDLE;\n      bit_count <= 0;\n      data_buffer <= 0;\n      done <= 0;\n    end else begin\n      state <= next_state;\n    end\n  end\n\n  // Combinational logic for next state and output control\n  always @(*) begin\n    next_state = state; // Default to stay in current state\n    done = 0; // Default done to 0\n    case (state)\n      IDLE: begin\n        if (in == 0) begin\n          next_state = RECEIVE;\n        end\n      end\n      RECEIVE: begin\n        if (bit_count == 7) begin // Check if 8 bits have been received\n          next_state = CHECK_STOP;\n        end\n      end\n      CHECK_STOP: begin\n        if (in == 1) begin\n          next_state = IDLE;\n          done = 1;\n        end\n      end\n      ERROR: begin\n        if (in == 1) begin\n          next_state = IDLE;\n        end\n      end\n    endcase\n  end\n\n  // Data reception logic\n  always @(posedge clk) begin\n    if (state == RECEIVE) begin\n      data_buffer <= {in, data_buffer[7:1]}; // Shift register operation\n      bit_count <= bit_count + 1;\n    end else begin\n      bit_count <= 0;\n    end\n  end\nendmodule"}
```

\*\*\*\*\*

>>>>>> EXECUTING FUNCTION verilog\_simulation\_tool...

user (to chat\_manager):

user (to chat\_manager):

\*\*\*\*\* Response from calling tool (call\_ecH4qKB5Hy8RR7nPhtw6wgZ) \*\*\*\*\*

[Compiled Success]

[Function Check Failed]

==Report start==

VCD info: dumpfile wave.vcd opened for output.

VCD warning: \$dumpvars: Package (\$unit) is not dumpable with VCD.

./test.sv:45: \$finish called at 4526 (1ps)

Hint: Output 'out\_byte' has no mismatches.

Hint: Output 'done' has 72 mismatches. First mismatch occurred at time 100.

Hint: Total mismatched samples is 72 out of 905 samples

Simulation finished at 4526 ps

Mismatches: 72 in 905 samples

==Report End==

Thought: input above output tool response into waveform\_trace\_tool to debug the failed signals starts with trace\_level=2!

\*\*\*\*\*

#### verilog\_engineer (to chat\_manager):

\*\*\*\*\* Suggested tool call (call\_IzFxSVZknlv7K9qKCIPPPph7): waveform\_trace\_tool \*\*\*\*\*

Arguments:

```
{"function_check_output": "[Compiled Success]\n[Function Check Failed]\n==Report start==\nVCD info: dumpfile wave.vcd opened for output.\nVCD warning: $dumpvars: Package ($unit) is not dumpable with VCD.\n./test.sv:45: $finish called at 4526 (1ps)\nHint: Output 'out_byte' has no mismatches.\nHint: Output 'done' has 72 mismatches. First mismatch occurred at time 100.\nHint: Total mismatched samples is 72 out of 905 samples\n\nSimulation finished at 4526 ps\nMismatches: 72 in 905 samples\n==Report End==", "trace_level": 2}
```

\*\*\*\*\*

>>>>>> EXECUTING FUNCTION waveform\_trace\_tool...

Creating new AST tree graph...

Generating LALR tables

WARNING: 183 shift/reduce conflicts

Get mismatched signal...

Hint: Total mismatched samples is 72 out of 905 samples

mismatches = 72

Trace graph signal...

```
deque([('reset', 'done'), ('in', 'done'), ('state', 'done')])
```

```
deque([('state', 'in'), ('next_state', 'state')])
```

```
deque([('next_state', 'state'), ('bit_count', 'next_state')])
```

Get table waveform...

```
['done_ref', 'in_ref', 'reset_ref'] ['done_dut', 'in_dut', 'reset_dut'] ['done', 'clk', 'in', 'reset']
```

data frame shape = 5 20

user (to chat\_manager):

user (to chat\_manager):

\*\*\*\*\* Response from calling tool (call\_LZFxSVZknlv7K9qKCiPPPh7) \*\*\*\*\*

[Verilog of DUT]:

```
```verilog
```

```
module TopModule (
```

```
    input logic clk,
```

```
    input logic in,
```

```
    input logic reset,
```

```
    output logic [7:0] out_byte,
```

```
    output logic done
```

```
);
```

```
    // State definitions
```

```
    localparam IDLE = 3'b000;
```

```
    localparam RECEIVE = 3'b001;
```

```
    localparam CHECK_STOP = 3'b010;
```

```
    localparam ERROR = 3'b011;
```

```
    // State register
```

```
    logic [2:0] state;
```

```
    logic [2:0] next_state;
```

```
    // Data bit counter
```

```
    logic [3:0] bit_count;
```

```
    // Data storage
```

```
    logic [7:0] data_buffer;
```

```
    // FSM logic to handle state transitions and outputs
```

```
    always @(posedge clk) begin
```

```
        if (reset) begin
```

```
            state <= IDLE;
```

```
            bit_count <= 0;
```

```
            data_buffer <= 0;
```

```
            done <= 0;
```

```
        end else begin
```

```
            state <= next_state;
```

```
        end
```

```
    end
```

```
    // Combinational logic for next state and output control
```

```
    always @(*) begin
```

```
        next_state = state; // Default to stay in current state
```

```
        done = 0; // Default done to 0
```

```
        case (state)
```

```
            IDLE: begin
```

```
                if (in == 0) begin
```

```
                    next_state = RECEIVE;
```

```
                end
```

```
            end
```

```
            RECEIVE: begin
```

```
                if (bit_count == 7) begin // Check if 8 bits have been received
```

```
                    next_state = CHECK_STOP;
```

```
                end
```

```

end
CHECK_STOP: begin
    if (in == 1) begin
        next_state = IDLE;
        done = 1;
        out_byte = data_buffer;
    end else begin
        next_state = ERROR;
    end
end
ERROR: begin
    if (in == 1) begin
        next_state = IDLE;
    end
end
endcase
end
// Data reception logic
always @(posedge clk) begin
    if (state == RECEIVE) begin
        data_buffer <= {in, data_buffer[7:1]}; // Shift register operation
        bit_count <= bit_count + 1;
    end else begin
        bit_count <= 0;
    end
end
endmodule
` `

```

[Signal Waveform]: <signal>\_tb is the given testbench signal and can not be changed! <signal>\_ref is the golden, and <signal>\_dut is the generated verilog file waveform. Check the mismatched signal waveform and its traced signals. The clock cycle (clk) is 10ns and toggles every 5ns.

'-' means unknown during simulation. If the '-' is the reason of mismatched signal, please check the reset and assignment block.

[Testbench Input Port Signal to Module]: clk, in, reset

[Traced Signals]: done, reset, in, state, next\_state, clk

[Table Waveform in hexadecimal format]

### First mismatched signals time(ns) Trace ###

| time(ns) | done_dut | done_ref | in_dut | in_ref | next_state_dut[2:0] | reset_dut | reset_ref | state_dut[2:0] |
|----------|----------|----------|--------|--------|---------------------|-----------|-----------|----------------|
| 0        | 0        | -        | 1      | 1      | -                   | 1         | 1         | -              |
| 5        | 0        | 0        | 0      | 0      | 1                   | 0         | 0         | 0              |
| 15       | 0        | 0        | 0      | 0      | 1                   | 0         | 0         | 1              |
| 85       | 0        | 0        | 0      | 0      | 2                   | 0         | 0         | 1              |
| 95       | 1        | 0        | 1      | 1      | 0                   | 0         | 0         | 2              |

### First mismatched signals time(ns) End ###

The values of mismatched signals at the first mismatched signal time above:

done\_dut: 1

done\_ref: 0

in\_dut: 1

in\_ref: 1

reset\_dut: 0

reset\_ref: 0

### Mismatched signals time(ns) Trace After the First Mismatch ###

| time(ns) | done_dut | done_ref | in_dut | in_ref | next_state_dut[2:0] | reset_dut | reset_ref | state_dut[2:0] |
|----------|----------|----------|--------|--------|---------------------|-----------|-----------|----------------|
| 0        | 0        | -        | 1      | 1      | -                   | 1         | 1         | -              |
| 5        | 0        | 0        | 0      | 0      | 1                   | 0         | 0         | 0              |
| 15       | 0        | 0        | 0      | 0      | 1                   | 0         | 0         | 1              |

|     |   |   |   |   |   |   |   |   |
|-----|---|---|---|---|---|---|---|---|
| 85  | 0 | 0 | 0 | 0 | 2 | 0 | 0 | 1 |
| 95  | 1 | 0 | 1 | 1 | 0 | 0 | 0 | 2 |
| 105 | 0 | 1 | 0 | 0 | 1 | 0 | 0 | 0 |
| 110 | 0 | 1 | 0 | 0 | 1 | 0 | 0 | 0 |
| 115 | 0 | 0 | 0 | 0 | 1 | 0 | 0 | 1 |
| 120 | 0 | 0 | 0 | 0 | 1 | 0 | 0 | 1 |

### Mismatched signals time(ns) Trace After the First Mismatch End ###

[Note] You can not change the [testbench input signal]: (clk, in, reset)! Modify the module implementation considering the input signals.

[Hint] Firstly, identify the time of mismatched signals, and only focus on the mismatched signals in the waveform firstly. Then, explain the related signals and their transitions in the waveform table. Don't correct signals without mismatch in the table waveforms. If the information is not enough for correct the functional error, try to trace more relevant signals using trace\_level > 2 for waveform\_trace\_tool. If you know how to correct the functional error, start to correct the code and run verilog\_simulation\_tool again.

\*\*\*\*\*

Removed 1 messages. Number of messages reduced from 5 to 4.

#### verilog\_engineer (to chat\_manager):

The waveform trace indicates that the `done` signal is set incorrectly at time 95 ns when it should remain 0. The issue occurs because the `done` signal is set to 1 in the `CHECK\_STOP` state without ensuring that all 8 bits have been correctly received and the stop bit is verified.

In the current implementation, the transition from `RECEIVE` to `CHECK\_STOP` occurs when `bit\_count` equals 7, which is incorrect because the bit count should reach 8 to ensure all bits are received. The `bit\_count` should be checked against 8 instead of 7 before transitioning to `CHECK\_STOP`.

Let's correct the code by adjusting the condition for transitioning from `RECEIVE` to `CHECK\_STOP` and ensure that `done` is set correctly based on the complete reception of the byte and the correct stop bit.

### Corrected Verilog Module

```

` ` `verilog
module TopModule (
    input logic clk,
    input logic in,
    input logic reset,
    output logic [7:0] out_byte,
    output logic done
);
    // State definitions
    localparam IDLE = 3'b000;
    localparam RECEIVE = 3'b001;
    localparam CHECK_STOP = 3'b010;
    localparam ERROR = 3'b011;
    // State register
    logic [2:0] state;
    logic [2:0] next_state;
    // Data bit counter
    logic [3:0] bit_count;
    // Data storage
    logic [7:0] data_buffer;
    // FSM logic to handle state transitions and outputs
    always @(posedge clk) begin
        if (reset) begin
            state <= IDLE;
            bit_count <= 0;
            data_buffer <= 0;
            done <= 0;
        end else begin
            state <= next_state;
        end
    end
end

```

```

// Combinational logic for next state and output control
always @(*) begin
    next_state = state; // Default to stay in current state
    done = 0; // Default done to 0
    case (state)
        IDLE: begin
            if (in == 0) begin
                next_state = RECEIVE;
            end
        end
        RECEIVE: begin
            if (bit_count == 8) begin // Check if 8 bits have been received
                next_state = CHECK_STOP;
            end
        end
        CHECK_STOP: begin
            if (in == 1) begin
                next_state = IDLE;
                done = 1;
                out_byte = data_buffer;
            end else begin
                next_state = ERROR;
            end
        end
        ERROR: begin
            if (in == 1) begin
                next_state = IDLE;
            end
        end
    endcase
end

// Data reception logic
always @(posedge clk) begin
    if (state == RECEIVE) begin
        data_buffer <= {in, data_buffer[7:1]}; // Shift register operation
        bit_count <= bit_count + 1;
    end else begin
        bit_count <= 0;
    end
end
endmodule
` ` `

```

Now, let's re-run the simulation tool to verify the corrected module.

\*\*\*\*\* Suggested tool call (call\_IzFxSVZknlv7K9qKCipPPph7): verilog\_simulation\_tool \*\*\*\*\*

Arguments:

```

{"completed_verilog": "module TopModule (\n  input logic clk,\n  input logic in,\n  input logic reset,\n  output logic [7:0] out_byte,\n  output logic done);\n\n  // State definitions\n  localparam IDLE = 3'b000;\n  localparam RECEIVE = 3'b001;\n  localparam CHECK_STOP = 3'b010;\n  localparam ERROR = 3'b011;\n\n  // State register\n  logic [2:0] state;\n  logic [2:0] next_state;\n\n  // Data bit counter\n  logic [3:0] bit_count;\n\n  // Data storage\n  logic [7:0] data_buffer;\n\n  // FSM logic to handle state transitions and outputs\n  always @(posedge clk) begin\n    if (reset) begin\n      state <= IDLE;\n      bit_count <= 0;\n      data_buffer <= 0;\n      done <= 0;\n    end else begin\n      state <= next_state;\n    end\n  end\n\n  // Combinational logic for next state and output control\n  always @(*) begin\n    next_state = state; // Default to stay in current state\n    done = 0; // Default done to 0\n    case (state)\n      IDLE: begin\n        if (in == 0) begin\n          next_state = RECEIVE;\n        end\n      end\n      RECEIVE: begin\n        if (bit_count == 8) begin // Check if 8 bits have been received\n          next_state = CHECK_STOP;\n        end\n      end\n      CHECK_STOP: begin\n        if (in == 1) begin\n          next_state = IDLE;\n          done = 1;\n          out_byte = data_buffer;\n        end else begin\n          next_state = ERROR;\n        end\n      end\n      ERROR: begin\n        if (in == 1) begin\n          next_state = IDLE;\n        end\n      end\n    endcase\n  end\nendmodule\n\n// Data

```

```

reception logic\n  always @(posedge clk) begin\n    if (state == RECEIVE) begin\n      data_buffer <= {in,\n      data_buffer[7:1]}; // Shift register operation\n      bit_count <= bit_count + 1;\n    end else begin\n      bit_count <=
0;\n    end\n  end\nendmodule"}

```

\*\*\*\*\*

>>>>>> EXECUTING FUNCTION verilog\_simulation\_tool...

user (to chat\_manager):

user (to chat\_manager):

\*\*\*\*\* Response from calling tool (call\_LZFxSVZknlv7K9qKCIPPPph7) \*\*\*\*\*

[Compiled Success]

[Function Check Failed]

==Report start==

VCD info: dumpfile wave.vcd opened for output.

VCD warning: \$dumpvars: Package (\$unit) is not dumpable with VCD.

./test.sv:45: \$finish called at 4526 (1ps)

Hint: Output 'out\_byte' has 38 mismatches. First mismatch occurred at time 110.

Hint: Output 'done' has 47 mismatches. First mismatch occurred at time 110.

Hint: Total mismatched samples is 57 out of 905 samples

Simulation finished at 4526 ps

Mismatches: 57 in 905 samples

==Report End==

Thought: input above output tool response into waveform\_trace\_tool to debug the failed signals starts with trace\_level=2!

\*\*\*\*\*

Removed 3 messages. Number of messages reduced from 7 to 4.

**verilog\_engineer (to chat\_manager):**

\*\*\*\*\* Suggested tool call (call\_MYioiyiyi7N5onObBsXGM5Whb): waveform\_trace\_tool \*\*\*\*\*

Arguments:

```

{"function_check_output": "[Compiled Success]\n[Function Check Failed]\n==Report start==\nVCD info: dumpfile
wave.vcd opened for output.\nVCD warning: $dumpvars: Package ($unit) is not dumpable with VCD.\n./test.sv:45: $finish
called at 4526 (1ps)\nHint: Output 'out_byte' has 38 mismatches. First mismatch occurred at time 110.\nHint: Output
'done' has 47 mismatches. First mismatch occurred at time 110.\nHint: Total mismatched samples is 57 out of 905
samples\n\nSimulation finished at 4526 ps\nMismatches: 57 in 905 samples\n==Report End==","trace_level":2}

```

\*\*\*\*\*

>>>>>> EXECUTING FUNCTION waveform\_trace\_tool...

Creating new AST tree graph...

Generating LALR tables

WARNING: 183 shift/reduce conflicts

Get mismatched signal...

Hint: Total mismatched samples is 57 out of 905 samples

mismatches = 57

Trace graph signal...

```

deque([('data_buffer', 'out_byte'), ('in', 'out_byte'), ('state', 'out_byte'), ('reset', 'done'), ('in', 'done'), ('state', 'done')])

```

```

deque([('reset', 'data_buffer'), ('in', 'data_buffer'), ('state', 'data_buffer'), ('state', 'in'), ('next_state', 'state'), ('reset', 'state'),
('next_state', 'state')])

```

```

deque([('next_state', 'state'), ('next_state', 'state'), ('bit_count', 'next_state'), ('bit_count', 'next_state')])

```

Get table waveform...

```

['done_ref', 'in_ref', 'out_byte_ref[7:0]', 'reset_ref'] ['done_dut', 'in_dut', 'out_byte_dut[7:0]', 'reset_dut'] ['out_byte', 'done',
'clk', 'in', 'reset']

```

Failed to transform to binary out\_byte\_dut[7:0] target line: -

data frame shape = 5 20

user (to chat\_manager):

user (to chat\_manager):

\*\*\*\*\* Response from calling tool (call\_MYioiyiyi7N5onObBsXGM5Whb) \*\*\*\*\*

[Verilog of DUT]:

```

` `` verilog

```

```

module TopModule (

```



```

input logic clk,
input logic in,
input logic reset,
output logic [7:0] out_byte,
output logic done
);
// State definitions
localparam IDLE = 3'b000;
localparam RECEIVE = 3'b001;
localparam CHECK_STOP = 3'b010;
localparam ERROR = 3'b011;
// State register
logic [2:0] state;
logic [2:0] next_state;
// Data bit counter
logic [3:0] bit_count;
// Data storage
logic [7:0] data_buffer;
// FSM logic to handle state transitions and outputs
always @(posedge clk) begin
    if (reset) begin
        state <= IDLE;
        bit_count <= 0;
        data_buffer <= 0;
        done <= 0;
    end else begin
        state <= next_state;
    end
end
// Combinational logic for next state and output control
always @(*) begin
    next_state = state; // Default to stay in current state
    done = 0; // Default done to 0
    case (state)
        IDLE: begin
            if (in == 0) begin
                next_state = RECEIVE;
            end
        end
        RECEIVE: begin
            if (bit_count == 8) begin // Check if 8 bits have been received
                next_state = CHECK_STOP;
            end
        end
        CHECK_STOP: begin
            if (in == 1) begin
                next_state = IDLE;
                done = 1;
                out_byte = data_buffer;
            end else begin
                next_state = ERROR;
            end
        end
        ERROR: begin
            if (in == 1) begin
                next_state = IDLE;
            end
        end
    end
end

```

```

        endcase
    end
    // Data reception logic
    always @(posedge clk) begin
        if (state == RECEIVE) begin
            data_buffer <= {in, data_buffer[7:1]}; // Shift register operation
            bit_count <= bit_count + 1;
        end else begin
            bit_count <= 0;
        end
    end
end
endmodule
`timescale 1ns/1ps

```

[Signal Waveform]: <signal>\_tb is the given testbench signal and can not be changed! <signal>\_ref is the golden, and <signal>\_dut is the generated verilog file waveform. Check the mismatched signal waveform and its traced signals. The clock cycle (clk) is 10ns and toggles every 5ns.

'-' means unknown during simulation. If the '-' is the reason of mismatched signal, please check the reset and assignment block.

[Testbench Input Port Signal to Module]: clk, in, reset

[Traced Signals]: out\_byte, done, data\_buffer, in, state, reset, next\_state, clk

[Table Waveform in hexadecimal format]

### First mismatched signals time(ns) Trace ###

| time(ns) | data_buffer_dut[7:0] | done_dut | done_ref | in_dut | in_ref | next_state_dut[2:0] | out_byte_dut[7:0] | out_byte_ref[7:0] |
|----------|----------------------|----------|----------|--------|--------|---------------------|-------------------|-------------------|
| 0        | -                    | 0        | -        | 1      | 1      | -                   | -                 | -                 |
| 5        | 0                    | 0        | 0        | 0      | 0      | 1                   | -                 | -                 |
| 15       | 0                    | 0        | 0        | 0      | 0      | 1                   | -                 | -                 |
| 95       | 0                    | 0        | 0        | 1      | 1      | 2                   | -                 | -                 |
| 105      | 80                   | 0        | 1        | 0      | 0      | 3                   | -                 | -                 |

### First mismatched signals time(ns) End ###

The values of mismatched signals at the first mismatched signal time above:

done\_dut: 0

done\_ref: 1

in\_dut: 0

in\_ref: 0

out\_byte\_dut[7:0]: -

out\_byte\_ref[7:0]: 0000

reset\_dut: 0

reset\_ref: 0

### Mismatched signals time(ns) Trace After the First Mismatch ###

| time(ns) | data_buffer_dut[7:0] | done_dut | done_ref | in_dut | in_ref | next_state_dut[2:0] | out_byte_dut[7:0] | out_byte_ref[7:0] |
|----------|----------------------|----------|----------|--------|--------|---------------------|-------------------|-------------------|
| 0        | -                    | 0        | -        | 1      | 1      | -                   | -                 | -                 |
| 5        | 0                    | 0        | 0        | 0      | 0      | 1                   | -                 | -                 |
| 15       | 0                    | 0        | 0        | 0      | 0      | 1                   | -                 | -                 |
| 95       | 0                    | 0        | 0        | 1      | 1      | 2                   | -                 | -                 |
| 105      | 80                   | 0        | 1        | 0      | 0      | 3                   | -                 | -                 |
| 115      | 80                   | 0        | 0        | 0      | 0      | 3                   | -                 | -                 |
| 120      | 80                   | 0        | 0        | 0      | 0      | 3                   | -                 | -                 |
| 125      | 80                   | 0        | 0        | 0      | 0      | 3                   | -                 | -                 |
| 130      | 80                   | 0        | 0        | 0      | 0      | 3                   | -                 | -                 |

### Mismatched signals time(ns) Trace After the First Mismatch End ###

[Note] You can not change the [testbench input signal]: (clk, in, reset)! Modify the module implementation considering the input signals.

[Hint] Firstly, identify the time of mismatched signals, and only focus on the mismatched signals in the waveform firstly. Then, explain the related signals and their transitions in the waveform table. Don't correct signals without mismatch

in the table waveforms. If the information is not enough for correct the functional error, try to trace more relevant signals using trace\_level > 2 for waveform\_trace\_tool. If you know how to correct the functional error, start to correct the code and run verilog\_simulation\_tool again.

\*\*\*\*\*

-----  
Removed 5 messages. Number of messages reduced from 9 to 4.

**verilog\_engineer (to chat\_manager):**

The waveform trace indicates that the `done` signal is set incorrectly at time 105 ns when it should be 1, but it remains 0. This issue arises because the transition from the `RECEIVE` state to the `CHECK\_STOP` state is based on the `bit\_count` reaching 8, but the `bit\_count` is incremented after the data is shifted into `data\_buffer`. This results in the `CHECK\_STOP` state being entered one clock cycle too late, causing the `done` signal to be set incorrectly.

To fix this, we need to adjust the condition for incrementing the `bit\_count` and transitioning to the `CHECK\_STOP` state. The `bit\_count` should be incremented before checking if it has reached 8, and the transition to `CHECK\_STOP` should occur when `bit\_count` equals 7 (since it will be incremented to 8 in the same cycle).

### Corrected Verilog Module

```
`verilog
module TopModule (
    input logic clk,
    input logic in,
    input logic reset,
    output logic [7:0] out_byte,
    output logic done
);
    // State definitions
    localparam IDLE = 3'b000;
    localparam RECEIVE = 3'b001;
    localparam CHECK_STOP = 3'b010;
    localparam ERROR = 3'b011;
    // State register
    logic [2:0] state;
    logic [2:0] next_state;
    // Data bit counter
    logic [3:0] bit_count;
    // Data storage
    logic [7:0] data_buffer;
    // FSM logic to handle state transitions and outputs
    always @(posedge clk) begin
        if (reset) begin
            state <= IDLE;
            bit_count <= 0;
            data_buffer <= 0;
            done <= 0;
        end else begin
            state <= next_state;
        end
    end
    // Combinational logic for next state and output control
    always @(*) begin
        next_state = state; // Default to stay in current state
        done = 0; // Default done to 0
        case (state)
            IDLE: begin
                if (in == 0) begin
                    next_state = RECEIVE;
                end
            end
            RECEIVE: begin
                if (bit_count == 7) begin // Check if 8 bits have been received
```

```

        next_state = CHECK_STOP;
    end
end
CHECK_STOP: begin
    if (in == 1) begin
        next_state = IDLE;
        done = 1;
        out_byte = data_buffer;
    end else begin
        next_state = ERROR;
    end
end
ERROR: begin
    if (in == 1) begin
        next_state = IDLE;
    end
end
endcase
end
// Data reception logic
always @(posedge clk) begin
    if (state == RECEIVE) begin
        bit_count <= bit_count + 1;
        data_buffer <= {in, data_buffer[7:1]}; // Shift register operation
    end else begin
        bit_count <= 0;
    end
end
endmodule
` ` `

```

Now, let's re-run the simulation tool to verify the corrected module.

\*\*\*\*\* Suggested tool call (call\_WgxSQT2R7NjyLQtvREVvaxAj): verilog\_simulation\_tool \*\*\*\*\*

Arguments:

```

{"completed_verilog": "module TopModule (\n  input logic clk,\n  input logic in,\n  input logic reset,\n  output logic [7:0] out_byte,\n  output logic done\n);\n\n  // State definitions\n  localparam IDLE = 3'b000;\n  localparam RECEIVE = 3'b001;\n  localparam CHECK_STOP = 3'b010;\n  localparam ERROR = 3'b011;\n\n  // State register\n  logic [2:0] state;\n  logic [2:0] next_state;\n\n  // Data bit counter\n  logic [3:0] bit_count;\n\n  // Data storage\n  logic [7:0] data_buffer;\n\n  // FSM logic to handle state transitions and outputs\n  always @(posedge clk) begin\n    if (reset) begin\n      state <= IDLE;\n      bit_count <= 0;\n      data_buffer <= 0;\n      done <= 0;\n    end else begin\n      state <= next_state;\n    end\n  end\n\n  // Combinational logic for next state and output control\n  always @(*) begin\n    next_state = state; // Default to stay in current state\n    done = 0; // Default done to 0\n    case (state)\n      IDLE: begin\n        if (in == 0) begin\n          next_state = RECEIVE;\n        end\n      end\n      RECEIVE: begin\n        if (bit_count == 7) begin // Check if 8 bits have been received\n          next_state = CHECK_STOP;\n        end\n        out_byte = data_buffer;\n        end else begin\n          next_state = ERROR;\n        end\n      end\n      ERROR: begin\n        if (in == 1) begin\n          next_state = IDLE;\n        end\n      end\n    endcase\n  end\n\n  // Data reception logic\n  always @(posedge clk) begin\n    if (state == RECEIVE) begin\n      bit_count <= bit_count + 1;\n      data_buffer <= {in, data_buffer[7:1]}; // Shift register operation\n    end else begin\n      bit_count <= 0;\n    end\n  end\nendmodule"}

```

\*\*\*\*\*

>>>>>> EXECUTING FUNCTION verilog\_simulation\_tool...

user (to chat\_manager):

user (to chat\_manager):

\*\*\*\*\* Response from calling tool (call\_WgxSQT2R7NjyLQtvREVvaxAj) \*\*\*\*\*

[Compiled Success]

[Function Check Failed]

==Report start==

```

VCD info: dumpfile wave.vcd opened for output.
VCD warning: $dumpvars: Package ($unit) is not dumpable with VCD.
./test.sv:45: $finish called at 4526 (1ps)
Hint: Output 'out_byte' has no mismatches.
Hint: Output 'done' has 72 mismatches. First mismatch occurred at time 100.
Hint: Total mismatched samples is 72 out of 905 samples
Simulation finished at 4526 ps
Mismatches: 72 in 905 samples
==Report End==
Thought: input above output tool response into waveform_trace_tool to debug the failed signals starts with trace_level=2!
*****
-----
Removed 7 messages. Number of messages reduced from 11 to 4.
verilog_engineer (to chat_manager):
***** Suggested tool call (call_e9LsUJLEQx1HvJpMaQtYPnAm): waveform_trace_tool *****
Arguments:
{"function_check_output": "[Compiled Success]\n[Function Check Failed]\n==Report start==\nVCD info: dumpfile
wave.vcd opened for output.\nVCD warning: $dumpvars: Package ($unit) is not dumpable with VCD.\n./test.sv:45: $finish
called at 4526 (1ps)\nHint: Output 'out_byte' has no mismatches.\nHint: Output 'done' has 72 mismatches. First
mismatch occurred at time 100.\nHint: Total mismatched samples is 72 out of 905 samples\n\nSimulation finished at
4526 ps\nMismatches: 72 in 905 samples\n==Report End==","trace_level":2}
*****
-----
>>>>>> EXECUTING FUNCTION waveform_trace_tool...
Creating new AST tree graph...
Generating LALR tables
WARNING: 183 shift/reduce conflicts
Get mismatched signal...
Hint: Total mismatched samples is 72 out of 905 samples
mismatches = 72
Trace graph signal...
deque([('reset', 'done'), ('in', 'done'), ('state', 'done')])
deque([('state', 'in'), ('next_state', 'state')])
deque([('next_state', 'state'), ('bit_count', 'next_state')])
Get table waveform...
['done_ref', 'in_ref', 'reset_ref'] ['done_dut', 'in_dut', 'reset_dut'] ['done', 'clk', 'in', 'reset']
data frame shape = 5 20
user (to chat_manager):
user (to chat_manager):
***** Response from calling tool (call_e9LsUJLEQx1HvJpMaQtYPnAm) *****
[Verilog of DUT]:
```verilog
module TopModule (
    input logic clk,
    input logic in,
    input logic reset,
    output logic [7:0] out_byte,
    output logic done
);
    // State definitions
    localparam IDLE = 3'b000;
    localparam RECEIVE = 3'b001;
    localparam CHECK_STOP = 3'b010;
    localparam ERROR = 3'b011;
    // State register
    logic [2:0] state;
    logic [2:0] next_state;
    // Data bit counter

```

```

logic [3:0] bit_count;
// Data storage
logic [7:0] data_buffer;
// FSM logic to handle state transitions and outputs
always @(posedge clk) begin
    if (reset) begin
        state <= IDLE;
        bit_count <= 0;
        data_buffer <= 0;
        done <= 0;
    end else begin
        state <= next_state;
    end
end
// Combinational logic for next state and output control
always @(*) begin
    next_state = state; // Default to stay in current state
    done = 0; // Default done to 0
    case (state)
        IDLE: begin
            if (in == 0) begin
                next_state = RECEIVE;
            end
        end
        RECEIVE: begin
            if (bit_count == 7) begin // Check if 8 bits have been received
                next_state = CHECK_STOP;
            end
        end
        CHECK_STOP: begin
            if (in == 1) begin
                next_state = IDLE;
                done = 1;
                out_byte = data_buffer;
            end else begin
                next_state = ERROR;
            end
        end
        ERROR: begin
            if (in == 1) begin
                next_state = IDLE;
            end
        end
    endcase
end
// Data reception logic
always @(posedge clk) begin
    if (state == RECEIVE) begin
        bit_count <= bit_count + 1;
        data_buffer <= {in, data_buffer[7:1]}; // Shift register operation
    end else begin
        bit_count <= 0;
    end
end
endmodule
` ``

```

[Signal Waveform]: <signal>\_tb is the given testbench signal and can not be changed! <signal>\_ref is the golden, and <signal>\_dut is the generated verilog file waveform. Check the mismatched signal waveform and its traced signals. The clock cycle (clk) is 10ns and toggles every 5ns.  
 '-' means unknown during simulation. If the '-' is the reason of mismatched signal, please check the reset and assignment block.

[Testbench Input Port Signal to Module]: clk, in, reset

[Traced Signals]: done, reset, in, state, next\_state, clk

[Table Waveform in hexadecimal format]

### First mismatched signals time(ns) Trace ###

|          | done_dut | done_ref | in_dut | in_ref | next_state_dut[2:0] | reset_dut | reset_ref | state_dut[2:0] |
|----------|----------|----------|--------|--------|---------------------|-----------|-----------|----------------|
| time(ns) |          |          |        |        |                     |           |           |                |
| 0        | 0        | -        | 1      | 1      | -                   | 1         | 1         | -              |
| 5        | 0        | 0        | 0      | 0      | 1                   | 0         | 0         | 0              |
| 15       | 0        | 0        | 0      | 0      | 1                   | 0         | 0         | 1              |
| 85       | 0        | 0        | 0      | 0      | 2                   | 0         | 0         | 1              |
| 95       | 1        | 0        | 1      | 1      | 0                   | 0         | 0         | 2              |

### First mismatched signals time(ns) End ###

The values of mismatched signals at the first mismatched signal time above:

done\_dut: 1

done\_ref: 0

in\_dut: 1

in\_ref: 1

reset\_dut: 0

reset\_ref: 0

### Mismatched signals time(ns) Trace After the First Mismatch ###

|          | done_dut | done_ref | in_dut | in_ref | next_state_dut[2:0] | reset_dut | reset_ref | state_dut[2:0] |
|----------|----------|----------|--------|--------|---------------------|-----------|-----------|----------------|
| time(ns) |          |          |        |        |                     |           |           |                |
| 0        | 0        | -        | 1      | 1      | -                   | 1         | 1         | -              |
| 5        | 0        | 0        | 0      | 0      | 1                   | 0         | 0         | 0              |
| 15       | 0        | 0        | 0      | 0      | 1                   | 0         | 0         | 1              |
| 85       | 0        | 0        | 0      | 0      | 2                   | 0         | 0         | 1              |
| 95       | 1        | 0        | 1      | 1      | 0                   | 0         | 0         | 2              |
| 105      | 0        | 1        | 0      | 0      | 1                   | 0         | 0         | 0              |
| 110      | 0        | 1        | 0      | 0      | 1                   | 0         | 0         | 0              |
| 115      | 0        | 0        | 0      | 0      | 1                   | 0         | 0         | 1              |
| 120      | 0        | 0        | 0      | 0      | 1                   | 0         | 0         | 1              |

### Mismatched signals time(ns) Trace After the First Mismatch End ###

[Note] You can not change the [testbench input signal]: (clk, in, reset)! Modify the module implementation considering the input signals.

[Hint] Firstly, identify the time of mismatched signals, and only focus on the mismatched signals in the waveform firstly. Then, explain the related signals and their transitions in the waveform table. Don't correct signals without mismatch in the table waveforms. If the information is not enough for correct the functional error, try to trace more relevant signals using trace\_level > 2 for waveform\_trace\_tool. If you know how to correct the functional error, start to correct the code and run verilog\_simulation\_tool again.

\*\*\*\*\*

Removed 9 messages. Number of messages reduced from 13 to 4.

**verilog\_engineer (to chat\_manager):**

The waveform trace reveals that the `done` signal is set incorrectly at 95 ns when it should be 0, but it is 1. This error occurs because the `done` signal is set to 1 in the `CHECK\_STOP` state when `in` is 1, but it does not account for the transition back to the `IDLE` state before setting `done` back to 0.

To correct this, we need to ensure that the `done` signal is only set to 1 for one clock cycle when the stop bit is correctly received and then reset to 0 in the next clock cycle as the FSM transitions back to the `IDLE` state.

### Corrected Verilog Module

```
```verilog
```

```
module TopModule (
```

```
    input logic clk,
```

```
    input logic in,
```

```

input logic reset,
output logic [7:0] out_byte,
output logic done
);
// State definitions
localparam IDLE = 3'b000;
localparam RECEIVE = 3'b001;
localparam CHECK_STOP = 3'b010;
localparam ERROR = 3'b011;
// State register
logic [2:0] state;
logic [2:0] next_state;
// Data bit counter
logic [3:0] bit_count;
// Data storage
logic [7:0] data_buffer;
// FSM logic to handle state transitions and outputs
always @(posedge clk) begin
    if (reset) begin
        state <= IDLE;
        bit_count <= 0;
        data_buffer <= 0;
        done <= 0;
    end else begin
        state <= next_state;
        if (state == CHECK_STOP && in == 1) begin
            done <= 1; // Set done only for one cycle when stop bit is correct
        end else begin
            done <= 0;
        end
    end
end
// Combinational logic for next state and output control
always @(*) begin
    next_state = state; // Default to stay in current state
    case (state)
        IDLE: begin
            if (in == 0) begin
                next_state = RECEIVE;
            end
        end
        RECEIVE: begin
            if (bit_count == 7) begin // Check if 8 bits have been received
                next_state = CHECK_STOP;
            end
        end
        CHECK_STOP: begin
            if (in == 1) begin
                next_state = IDLE;
                out_byte = data_buffer;
            end else begin
                next_state = ERROR;
            end
        end
        ERROR: begin
            if (in == 1) begin
                next_state = IDLE;
            end
        end
    end
end

```



```

        end
    endcase
end
// Data reception logic
always @(posedge clk) begin
    if (state == RECEIVE) begin
        bit_count <= bit_count + 1;
        data_buffer <= {in, data_buffer[7:1]}; // Shift register operation
    end else begin
        bit_count <= 0;
    end
end
endmodule
` ` `

```

Now, let's re-run the simulation tool to verify the corrected module.

\*\*\*\*\* Suggested tool call (call\_azcbF1Igu934nD80wolnesYr): verilog\_simulation\_tool \*\*\*\*\*

Arguments:

```

{"completed_verilog": "module TopModule (\n  input logic clk,\n  input logic in,\n  input logic reset,\n  output logic [7:0] out_byte,\n  output logic done);\n\n  // State definitions\n  localparam IDLE = 3'b000;\n  localparam RECEIVE = 3'b001;\n  localparam CHECK_STOP = 3'b010;\n  localparam ERROR = 3'b011;\n\n  // State register\n  logic [2:0] state;\n  logic [2:0] next_state;\n\n  // Data bit counter\n  logic [3:0] bit_count;\n\n  // Data storage\n  logic [7:0] data_buffer;\n\n  // FSM logic to handle state transitions and outputs\n  always @(posedge clk) begin\n    if (reset) begin\n      state <= IDLE;\n      bit_count <= 0;\n      data_buffer <= 0;\n      done <= 0;\n    end else begin\n      state <= next_state;\n      if (state == CHECK_STOP && in == 1) begin\n        done <= 1; // Set done only for one cycle when stop bit is correct\n      end else begin\n        done <= 0;\n      end\n    end\n\n    // Combinational logic for next state and output control\n    always @(*) begin\n      next_state = state; // Default to stay in current state\n      case (state)\n        IDLE: begin\n          if (in == 0) begin\n            next_state = RECEIVE;\n          end\n        end\n        RECEIVE: begin\n          if (bit_count == 7) begin // Check if 8 bits have been received\n            next_state = CHECK_STOP;\n          end\n        end\n        CHECK_STOP: begin\n          if (in == 1) begin\n            next_state = IDLE;\n          end\n        end\n        ERROR: begin\n          if (in == 1) begin\n            next_state = IDLE;\n          end\n        end\n      endcase\n    end\n\n    // Data reception logic\n    always @(posedge clk) begin\n      if (state == RECEIVE) begin\n        bit_count <= bit_count + 1;\n        data_buffer <= {in, data_buffer[7:1]}; // Shift register operation\n      end else begin\n        bit_count <= 0;\n      end\n    end\n  end\nendmodule"}

```

\*\*\*\*\*

>>>>>> EXECUTING FUNCTION verilog\_simulation\_tool...

user (to chat\_manager):

user (to chat\_manager):

\*\*\*\*\* Response from calling tool (call\_azcbF1Igu934nD80wolnesYr) \*\*\*\*\*

[Compiled Success]

[Function Check Success]

VCD info: dumpfile wave.vcd opened for output.

VCD warning: \$dumpvars: Package (\$unit) is not dumpable with VCD.

./test.sv:45: \$finish called at 4526 (1ps)

Hint: Output 'out\_byte' has no mismatches.

Hint: Output 'done' has no mismatches.

Hint: Total mismatched samples is 0 out of 905 samples

Simulation finished at 4526 ps

Mismatches: 0 in 905 samples

\*\*\*\*\*

Removed 11 messages. Number of messages reduced from 15 to 4.

**verilog\_engineer (to chat\_manager):**

TERMINATE
